# Supplementary material for: Shortcut to Chemically Accurate Quantum Computing via Density-based Basis-set Correction
Source: arXiv:2405.11567 ancillary file (2024-10-05)
Supplement: Supplementary file 1 [file Shortcut-SI-V2.pdf]

# Supplementary Information: Shortcut to chemically accurate quantum computing via density-based basis-set correction


Diata Traore,[1,2] Olivier Adjoua,[1] Cesar Feniou,[2,1] Ioanna-Maria Lygatsika,[3,1,*] Yvon Maday,[3,4] Evgeny Posenitskiy,[2] Kerstin Hammernik,[5] Alberto Peruzzo,[2] Julien Toulouse,[1,4] Emmanuel Giner,[1] and Jean-Philip Piquemal[1,2,†]

[1]*Sorbonne Université, LCT, UMR 7616 CNRS, 75005 Paris, France*
[2]*Qubit Pharmaceuticals, Advanced Research Department, 75014 Paris, France*
[3]*Sorbonne Université, LJLL, UMR 7598 CNRS, 75005 Paris, France*
[4]*Institut Universitaire de France, 75005 Paris, France*
[5]*NVIDIA Corporation, Santa Clara, CA, USA*


## I. MAPPING QUANTUM CHEMISTRY TO QUANTUM COMPUTERS AND QUANTUM SOLVER

In a given spin-orbital basis set $\mathcal{B}$, the molecular electronic Hamiltonian can be expressed in second-quantization as

$$\hat{H} = \sum_{p,q} h_{pq} \hat{a}_p^\dagger \hat{a}_q + \sum_{p,q,r,s} w_{pqrs} \hat{a}_p^\dagger \hat{a}_q^\dagger \hat{a}_s \hat{a}_r, \tag{1}$$

where the indices $p, q, r, s$ run over the spin-orbitals, $\hat{a}_p$ and $\hat{a}_p^\dagger$ are the $p^{\text{th}}$ fermionic annihilation and creation operators, and $h_{pq}$ and $w_{pqrs}$ are the one-electron and two-electron integrals. The Jordan-Wigner and Bravyi-Kitaev transforms [1, 2] are usually employed to map annihilation and creation operators to tensor products involving Pauli matrices, enabling the representation of the second-quantized Hamiltonian $\hat{H}$ on a quantum computer, with each qubit encoding a spin-orbital of the system. The molecular Hamiltonian $\hat{H}$ now expressed as linear combination of Pauli products, various quantum algorithms such as the Variational Quantum Eigensolver (VQE) [3] and Quantum Phase Estimation (QPE) [4, 5] can compute the ground state of this molecular Hamiltonian [6–8]. In this paper, a VQE-inspired algorithm is used. The VQE minimizes the Hamiltonian's expectation value with respect to a parameterized ansatz wave function, in a classical-quantum hybrid approach. The challenge is constructing an ansatz wave function balancing accuracy with a shallow quantum-circuit representation for NISQ devices. To address such a challenge, the adaptive derivative-assembled pseudo-Trotter variational quantum eigensolver (ADAPT-VQE) [9] has emerged as a standard, by proposing an ansatz that is dynamically grown through an iterative process, resulting in an increased accuracy with shallower circuits than traditional VQE ansatze, for which the structure is predetermined before simulations. The general workflow of the ADAPT-VQE algorithm is as explained in Ref. [10].

In the present study, we use the Qubit-Excitation-Based pool of operators, which is considered a standard [11]. Note that one issue of ADAPT-VQE is linked to its classical optimization procedure that can encounter barren plateaus generating very large numbers of parameters and therefore limiting practical convergence. In such cases, a variant of ADAPT-VQE can be used: the Overlap-ADAPT-VQE [12] that allows one to grow wave functions by maximizing their overlap with an intermediate target wave function. That way, when barren plateaus are encountered, Overlap-ADAPT-VQE can reduce the number of optimization parameters and produce an ultra-compact ansatz suitable for high-accuracy initialization of a new ADAPT procedure able to converge faster to full configuration interaction (FCI).


* Present address: CEA, DAM, DIF, F-91297 Arpajon, France; and Université Paris-Saclay, LMCE, 91680 Bruyères-le-Châtel, France
† jean-philip.piquemal@sorbonne-universite.fr

# II. DATA

## A. Geometries

TABLE I: Geometries (in Å) of the molecular systems studied present in the paper.

| System | | x | y | z |
|---|---|---|---|---|
| $N_2$ | N | 0. | 0. | 0. |
| | N | 0. | 0. | 1.0977 |
| $H_2O$ | O | 0. | 0. | 0.1173 |
| | H | 0. | 0.7572 | -0.4692 |
| | H | 0. | -0.7572 | -0.4692 |
| LiH | Li | 0. | 0. | 0. |
| | H | 0. | 0. | 1.5949 |
| $H_n$ | H | 0. | 0. | 0.0 |
| | H | 0. | 0. | 0.8 |
| | ... | | | |
| | H | 0. | 0 | $0.8(n-1)$ |

## B. Total ground-state energies with standard basis sets

TABLE II: Ground-state energies (in Ha) for He, Be, FH, LiH, and $H_2O$ at the HF, near-FCI (CIPSI+PT2), ADAPT-VQE (denoted as ADAPT), non-self-consistent basis-set corrected near-FCI (denoted as FCI+PBE+ΔHF), and self-consistent basis-set corrected ADAPT-VQE without the HF basis-set correction (denoted as SC(ADAPT+PBE)). The values of the PBE-based correlation basis-set correction and of the HF basis-set correction are also given. The frozen-core approximation is used for Be, FH, LiH, and $H_2O$. The CBS limits are estimated by two-point extrapolations from cc-pVQZ and cc-pV5Z calculations. The number of iterations for the ADAPT-VQE calculations are given in bracket.

| He | $N_{\text{qubits}}$ | HF | ΔHF | PBE | FCI | FCI+PBE+ΔHF | ADAPT | SC(ADAPT+PBE) |
|---|---|---|---|---|---|---|---|---|
| STO-3G | 2 | -2.80778 | -0.05384 | -0.03182 | -2.80778 | -2.89344 | - | - |
| pc-seg0 | 4 | -2.83405 | -0.02757 | -0.01812 | -2.84979 | -2.89548 | -2.84979 [3] | -2.86791 |
| 6-31G | 4 | -2.85516 | -0.00646 | -0.01950 | -2.87016 | -2.89612 | -2.87016 [3] | -2.88960 |
| cc-pVDZ | 10 | -2.85516 | -0.00646 | -0.01168 | -2.88759 | -2.90573 | -2.88759 [6] | -2.89927 |
| cc-pVTZ | 28 | -2.86115 | -0.00047 | -0.00420 | -2.90023 | -2.9049 | - | - |
| cc-pVQZ | 60 | -2.86151 | -0.00011 | -0.00167 | -2.90241 | -2.90419 | - | - |
| cc-pV5Z | 110 | -2.86162 | 0 | -0.00084 | -2.90315 | -2.90399 | - | - |
| CBS | - | - | - | - | -2.90392 | - | - | - |
| Be | $N_{\text{qubits}}$ | HF | ΔHF | PBE | FCI | FCI+PBE+ΔHF | ADAPT | SC(ADAPT+PBE) |
| STO-3G | 8 | -14.35188 | -0.22113 | -0.00789 | -14.40332 | -14.63234 | -14.40333 [3] | -14.41120 |
| pc-seg0 | 10 | -14.53608 | -0.03693 | -0.00439 | -14.57712 | -14.61844 | -14.57712 [6] | -14.58160 |
| 6-31G | 16 | -14,56676 | 1,456,661 | -0.00360 | -14.61274 | 1,456,647 | -14.61274 [19][a] | -14.61641 |
| cc-pVDZ | 26 | -14.57234 | -0.00067 | -0.00187 | -14.61684 | -14.61938 | -14.61684 [24] | -14.61884 |
| cc-pVTZ | 58 | -14.57287 | -0.00014 | -0.00082 | -14.61842 | -14.61938 | - | - |
| cc-pVQZ | 108 | -14.57297 | -0.00004 | -0.00038 | -14.61895 | -14.61937 | - | - |
| cc-pV5Z | 180 | -14.57301 | 0 | -0.00021 | -14.61908 | -14.61929 | - | - |
| CBS | - | - | - | - | -14.61921 | - | - | - |
| LiH | $N_{\text{qubits}}$ | HF | ΔHF | PBE | FCI | FCI+PBE+ΔHF | ADAPT | SC(ADAPT+PBE) |
| STO-3G | 10 | -7.86203 | -0.12529 | -0.01413 | -7.88218 | -8.0216 | -7.88218 [10] | -7.89590 |
| pc-seg0 | 14 | -7.96337 | -0.02395 | -0.01066 | -7.98139 | -8.016 | -7.98139 [26] | -7.99166 |
| 6-31G | 20 | -7.97927 | -0.00805 | -0.01063 | -7.99800 | -8.01668 | -7.99800 [47][b] | -8.00806 |
| VQZ-4 | 10 | -7.97603 | -0.01129 | -0.01344 | -7.99281 | -8.01754 | -7.99281 [10] | -8.00557 |
| V5Z-4 | 10 | -7.97604 | -0.01128 | -0.01343 | -7.99287 | -8.01758 | -7.99287 [10] | -8.00562 |
| V5Z-7 | 16 | -7.98198 | -0.00534 | -0.01383 | -7.99793 | -8.0171 | -7.99793 [27] | -8.01658 |
| V5Z-10 | 28 | -7.98326 | -0.00406 | -0.00867 | -8.01302 | -8.02575 | -8.01302 [91] | -8.02134 |
| cc-pVDZ | 36 | -7.98373 | -0.00359 | -0.00418 | -8.01438 | -8.02215 | - | - |
| cc-pVTZ | 86 | -7.98665 | -0.00067 | -0.00145 | -8.02234 | -8.02446 | - | - |
| cc-pVQZ | 190 | -7.98718 | -0.00014 | -0.00063 | -8.02386 | -8.02463 | - | - |
| cc-pV5Z | 290 | -7.98732 | 0 | -0.00035 | -8.02433 | -8.02468 | - | - |
| CBS | - | - | - | - | -8.02482 | - | - | - |
| $H_2O$ | $N_{\text{qubits}}$ | HF | ΔHF | PBE | FCI | FCI+PBE+ΔHF | ADAPT | SC(ADAPT+PBE) |
| STO-3G | 12 | -74.96302 | -1.10403 | -0.185798 | -75.01250 | -76.302328 | -75.01250 [63] | -75.19788 |
| pc-seg0 | 24 | -75.77425 | -0.2928 | -0.135581 | -75.90855 | -76.336931 | -75.90842 [1000][c] | -76.03999 |
| 6-31G | 24 | -75.98397 | -0.08308 | -0.07738 | -76.11995 | -76.28041 | -76.11989 [1000][d] | -76.23717 |
| V5Z-10 | 24 | -76.01618 | -0.05087 | -0.15209 | -76.12626 | -76.32922 | -76.12409 [1000] | -76.27418 |
| V5Z-11 | 30 | -76.01756 | -0.04948 | -0.13591 | -76.15902 | -76.34441 | -76.15165 [541] | -76.28622 |
| cc-pVDZ | 46 | -76.02677 | -0.04028 | -0.07406 | -76.24165 | -76.35599 | - | - |
| cc-pVTZ | 114 | -76.05713 | -0.00992 | -0.03063 | -76.33250 | -76.37305 | - | - |
| cc-pVQZ | 228 | -76.06479 | -0.00226 | -0.01471 | -76.35985 | -76.37682 | - | - |
| cc-pV5Z | 400 | -76.06705 | 0 | -0.00801 | -76.36877 | -76.37678 | - | - |
| CBS | - | - | - | - | -76.37812 | - | - | - |
| $N_2$ | $N_{\text{qubits}}$ | HF | ΔHF | PBE | FCI | FCI+PBE+ΔHF | ADAPT | SC(ADAPT+PBE) |
| STO-3G | 16 | -107.49589 | -1.49687 | -0.21692 | -107.65253 | -109.36632 | -107.65251 [386] | -107.86974 |
| V5Z-6 | 16 | -108.74518 | -0.24758 | -0.20925 | -108.88869 | -109.34552 | -108.88869 [759] | -109.09850 |
| cc-pVDZ | 52 | -108.95412 | -0.03864 | -0.08984 | -109.27698 | -109.40546 | - | - |
| cc-pVTZ | 116 | -108.98347 | -0.00929 | -0.03695 | -109.37527 | -109.42151 | - | - |
| cc-pVQZ | 216 | -108.99108 | -0.00168 | -0.01788 | -109.40558 | -109.42514 | - | - |
| cc-pV5Z | 360 | -108.99276 | 0 | -0.00996 | -109.41505 | -109.42501 | - | - |
| CBS | - | - | - | - | -109.42498 | - | - | - |

[a] From the 19th iteration, the ADAPT-VQE iterations kept choosing the same operator, thus the energy stops varying from iteration 19.
[b] From the 47th iteration, the ADAPT-VQE iterations kept choosing the same operator, thus the energy stops varying from iteration 47.
[c] Initial state has 10879 determinants.
[d] Initial state has 14668 determinants.

TABLE III: Ground-state energies (in Ha) for hydrogen chains with atomic distances of 0.8 Å at the HF, near-FCI (CIPSI+PT2), ADAPT-VQE (denoted as ADAPT), non-self-consistent basis-set corrected near-FCI (denoted as FCI+PBE+ΔHF), and self-consistent basis-set corrected ADAPT-VQE without the HF basis-set correction (denoted as SC(ADAPT+PBE)). The values of the PBE-based correlation basis-set correction and of the HF basis-set correction are also given. The CBS limits are estimated by two-point extrapolations from cc-pVQZ and cc-pV5Z calculations. The number of iterations for the ADAPT-VQE calculations are given in bracket.

| $H_2$ | $N_{\text{qubits}}$ | HF | ΔHF | PBE | FCI | FCI+PBE+ΔHF | ADAPT | SC(ADAPT+PBE) |
|---|---|---|---|---|---|---|---|---|
| STO-3G | 4 | -1.11085 | -0.02004 | -0.02187 | -1.13415 | -1.17606 | -1.13415 [1] | -1.15590 |
| 6-31G | 8 | -1.12371 | -0.00717 | -0.01191 | -1.15003 | -1.16911 | -1.15003 [7] | -1.16196 |
| cc-pVDZ | 20 | -1.12700 | -0.00388 | -0.00576 | -1.16275 | -1.17239 | -1.16275 [21] | -1.16858 |
| V5Z-8 | 24 | -1.12938 | -0.00150 | -0.00552 | -1.16613 | -1.17315 | -1.16613 [35] | -1.17170 |
| cc-pVTZ | 56 | -1.13029 | -0.00059 | -0.00177 | -1.17041 | -1.17277 | - | - |
| cc-pVQZ | 120 | -1.13075 | -0.00014 | -0.00074 | -1.17182 | -1.17270 | - | - |
| cc-pV5Z | 220 | -1.13089 | 0 | -0.00037 | -1.17223 | -1.17260 | - | - |
| CBS | - | - | - | - | -1.17265 | - | - | - |

| $H_4$ | $N_{\text{qubits}}$ | HF | ΔHF | PBE | FCI | FCI+PBE+ΔHF | ADAPT | SC(ADAPT+PBE) |
|---|---|---|---|---|---|---|---|---|
| STO-3G | 8 | -2.12139 | -0.05672 | -0.04299 | -2.16756 | -2.26727 | -2.16756 [19] | -2.21040 |
| cc-pVDZ | 40 | -2.16785 | -0.01026 | -0.01188 | -2.24884 | -2.27098 | - | - |
| cc-pVTZ | 112 | -2.17696 | -0.00115 | -0.00371 | -2.26848 | -2.27333 | - | - |
| cc-pVQZ | 240 | -2.17782 | -0.00029 | -0.00157 | -2.27134 | -2.27320 | - | - |
| cc-pV5Z | 438 | -2.17811 | 0 | -0.00078 | -2.27222 | -2.27299 | - | - |
| CBS | - | - | - | - | -2.27315 | - | - | - |

| $H_6$ | $N_{\text{qubits}}$ | HF | ΔHF | PBE | FCI | FCI+PBE+ΔHF | ADAPT | SC(ADAPT+PBE) |
|---|---|---|---|---|---|---|---|---|
| STO-3G | 12 | -3.13461 | -0.09203 | -0.04299 | -3.20441 | -3.33943 | -3.20441 [200] | -3.26858 |
| 6-31G | 24 | -3.20987 | -0.01677 | -0.02653 | -3.29582 | -3.33912 | - | - |
| cc-pVDZ | 60 | -3.20989 | -0.01675 | -0.01801 | -3.33763 | -3.37239 | - | - |
| cc-pVTZ | 168 | -3.22483 | -0.00181 | -0.00566 | -3.36939 | -3.37686 | - | - |
| cc-pVQZ | 360 | -3.22619 | -0.00045 | -0.00241 | -3.37379 | -3.37665 | - | - |
| cc-pV5Z | 650 | -3.22664 | 0 | -0.00120 | - | - | - | - |
| CBS | - | - | - | - | - | - | - | - |

| $H_8$ | $N_{\text{qubits}}$ | HF | ΔHF | PBE | FCI | FCI+PBE+ΔHF | ADAPT | SC(ADAPT+PBE) |
|---|---|---|---|---|---|---|---|---|
| STO-3G | 16 | -4.14962 | -0.1259 | -0.08573 | -4.24339 | -4.45502 | -4.24320 [1000] | -4.32764 |
| 6-31G | 32 | -4.25325 | -0.02227 | -0.05509 | -4.37032 | -4.44768 | -4.35752 [685] | -4.41275 |
| cc-pVDZ | 80 | -4.25244 | -0.02308 | -0.02419 | -4.42756 | -4.47483 | - | - |
| cc-pVTZ | 222 | -4.27304 | -0.00248 | -0.00762 | -4.47121 | -4.48131 | - | - |
| cc-pVQZ | 474 | -4.27490 | -0.00062 | -0.00327 | - | - | - | - |
| cc-pV5Z | 864 | -4.27552 | 0 | - | - | - | - | - |
| CBS | - | - | - | - | - | - | - | - |

| $H_{10}$ | $N_{\text{qubits}}$ | HF | ΔHF | PBE | FCI | FCI+PBE+ΔHF | ADAPT | SC(ADAPT+PBE) |
|---|---|---|---|---|---|---|---|---|
| STO-3G | 20 | -5.16558 | -0.15903 | -0.10712 | -5.28355 | -5.5497 | - | - |
| cc-pVDZ | 100 | -5.29511 | -0.0295 | -0.03040 | -5.51771 | -5.57761 | - | - |
| cc-pVTZ | 278 | -5.32146 | -0.00315 | -0.00959 | -5.57298 | -5.58572 | - | - |
| cc-pVQZ | 590 | -5.32381 | -0.0008 | -0.00412 | - | - | - | - |
| cc-pV5Z | 1074 | -5.32461 | 0 | - | - | - | - | - |
| CBS | - | -5.32545 | - | - | - | - | - | - |

### C. Total ground-state energies with SABS

The target SABS sizes vary from minimal basis size (STO-3G) to the full size of the original AO basis set.

TABLE IV: [1/2] Ground-state energies (in Ha) of the $H_2$ molecule calculated by HF, near-FCI (CIPSI+PT2), and self-consistent basis-set corrected near-FCI without and with the HF basis-set correction (denoted as SC(FCI+PBE) and SC(FCI+PBE)+$\Delta$HF, respectively). VXZ-Y corresponds to the cc-pVXZ basis transformed to a basis of Y AO functions following the SABS building procedure. The notation VXZ-[$Y_n$-$Y_{n+a}$] means that the values are the same for the basis sets VXY-$Y_n$, VXY-$Y_{n+1}$, ..., VXY-$Y_{n+a-1}$, and VXY-$Y_{n+a}$. The FCI/CBS limit is -1.13103 Ha.

| $H_2$ | Basis set | # active MOs | HF | FCI | SC(FCI+PBE) | SC(FCI+PBE)+$\Delta$HF |
|---|---|---|---|---|---|---|
| | VDZ-[2-3] | 2 | -1.09635 | -1.11372 | -1.13412 | -1.16880 |
| | VDZ-[4-5] | 4 | -1.12286 | -1.14810 | -1.16186 | -1.17002 |
| | VDZ-6 | 10 | -1.12700 | -1.16275 | -1.16857 | -1.17260 |
| | VTZ-[2-3] | 2 | -1.09723 | -1.11461 | -1.13498 | -1.16878 |
| | VTZ-[4-5] | 4 | -1.12226 | -1.14639 | -1.16134 | -1.17010 |
| | VTZ-[6-7] | 6 | -1.12513 | -1.15191 | -1.16293 | -1.16883 |
| | VTZ-[8-9] | 12 | -1.12949 | -1.16278 | -1.16649 | -1.16802 |
| | VTZ-[10-12] | 18 | -1.13027 | -1.16890 | -1.17188 | -1.17263 |
| | VTZ-13 | 18 | -1.13027 | -1.16890 | -1.17188 | -1.17263 |
| | VTZ-14 | 28 | -1.13029 | -1.17040 | -1.17215 | -1.17289 |
| | VQZ-[2-3] | 2 | -1.09751 | -1.11491 | -1.13527 | -1.16879 |
| | VQZ-4 | 4 | -1.12096 | -1.14421 | -1.16002 | -1.17008 |
| | VQZ-[5-7] | 6 | -1.12552 | -1.15237 | -1.16356 | -1.16906 |
| | VQZ-[8-9] | 12 | -1.13005 | -1.16638 | -1.17068 | -1.17166 |
| | VQZ-10 | 18 | -1.13019 | -1.16856 | -1.17246 | -1.17330 |
| | VQZ-[11-12] | 20 | -1.13040 | -1.16907 | -1.17252 | -1.17314 |
| | VQZ-[13-15] | 26 | -1.13067 | -1.16987 | -1.17214 | -1.17250 |
| | VQZ-[16-19] | 36 | -1.13074 | -1.17092 | -1.17218 | -1.17246 |
| | VQZ-20 | 46 | -1.13074 | -1.17158 | -1.17258 | -1.17286 |
| | VQZ-21 | 46 | -1.13074 | -1.17158 | -1.17259 | -1.17287 |
| | VQZ-22 | 60 | -1.13074 | -1.17182 | -1.17257 | -1.17285 |
| | V5Z-2 | 2 | -1.09759 | -1.11499 | -1.13535 | -1.16879 |
| | V5Z-[3-6] | 4 | -1.12106 | -1.14572 | -1.15779 | -1.16776 |
| | V5Z-7 | 10 | -1.12579 | -1.16014 | -1.16560 | -1.17083 |
| | V5Z-8 | 12 | -1.12938 | -1.16613 | -1.17170 | -1.17335 |
| | V5Z-9 | 14 | -1.13016 | -1.16720 | -1.17199 | -1.17286 |
| | V5Z-[10-12] | 20 | -1.13018 | -1.16816 | -1.17246 | -1.17331 |
| | V5Z-[13-15] | 26 | -1.13078 | -1.16986 | -1.17232 | -1.17256 |
| | V5Z-16 | 28 | -1.13079 | -1.17006 | -1.17234 | -1.17257 |
| | V5Z-17 | 28 | -1.13079 | -1.17006 | -1.17232 | -1.17255 |
| | V5Z-18 | 38 | -1.13081 | -1.17101 | -1.17290 | -1.17312 |
| | V5Z-19 | 48 | -1.13085 | -1.17167 | -1.17290 | -1.17308 |
| | V5Z-20 | 54 | -1.13087 | -1.17175 | -1.17274 | -1.17290 |
| | V5Z-21 | 54 | -1.13087 | -1.17175 | -1.17274 | -1.17289 |
| | V5Z-22 | 54 | -1.13087 | -1.17175 | -1.17270 | -1.17286 |
| | V5Z-[23-26] | 68 | -1.13087 | -1.17194 | -1.17281 | -1.17296 |
| | V5Z-[27-28] | 78 | -1.13088 | -1.17205 | -1.17268 | -1.17283 |
| | V5Z-[29-31] | 92 | -1.13088 | -1.17216 | -1.17260 | -1.17275 |
| | V5Z-32 | 110 | -1.13088 | -1.17222 | -1.17252 | -1.17267 |

TABLE V: [2/2] Ground-state energies (in Ha) of the $H_2$ molecule calculated by HF, near-FCI (CIPSI+PT2), and self-consistent basis-set corrected near-FCI without and with the HF basis-set correction (denoted as SC(FCI+PBE) and SC(FCI+PBE)+$\Delta$HF, respectively). VXZ-Y corresponds to the cc-pVXZ basis transformed to a basis of Y AO functions following the SABS building procedure. The notation VXZ-[$Y_n$-$Y_{n+a}$] means that the values are the same for the basis sets VXY-$Y_n$, VXY-$Y_{n+1}$, ..., VXY-$Y_{n+a-1}$, and VXY-$Y_{n+a}$. The FCI/CBS limit is -1.13103 Ha.

| $H_2$ | Basis set | # active MOs | HF | FCI | SC(FCI+PBE) | SC(FCI+PBE)+$\Delta$HF |
|---|---|---|---|---|---|---|
| | V6Z-[2-3] | 2 | -1.09760 | -1.11500 | -1.13536 | -1.16879 |
| | V6Z-4 | 4 | -1.12438 | -1.15020 | -1.16311 | -1.16976 |
| | V6Z-5 | 10 | -1.12791 | -1.16391 | -1.17072 | -1.17383 |
| | V6Z-[6-8] | 12 | -1.12829 | -1.16455 | -1.17064 | -1.17337 |
| | V6Z-[9-10] | 18 | -1.12832 | -1.16503 | -1.17045 | -1.17315 |
| | V6Z-11 | 20 | -1.12979 | -1.16704 | -1.17220 | -1.17344 |
| | V6Z-12 | 26 | -1.13068 | -1.16963 | -1.17239 | -1.17273 |
| | V6Z-[13-17] | 28 | -1.13077 | -1.16993 | -1.17243 | -1.17268 |
| | V6Z-18 | 38 | -1.13081 | -1.17129 | -1.17301 | -1.17323 |
| | V6Z-19 | 52 | -1.13081 | -1.17151 | -1.17293 | -1.17315 |
| | V6Z-20 | 52 | -1.13081 | -1.17151 | -1.17294 | -1.17316 |
| | V6Z-21 | 54 | -1.13082 | -1.17156 | -1.17292 | -1.17313 |
| | V6Z-22 | 54 | -1.13082 | -1.17156 | -1.17294 | -1.17314 |
| | V6Z-23 | 54 | -1.13082 | -1.17156 | -1.17293 | -1.17314 |
| | V6Z-24 | 60 | -1.13087 | -1.17173 | -1.17276 | -1.17291 |
| | V6Z-25 | 70 | -1.13088 | -1.17181 | -1.17285 | -1.17299 |
| | V6Z-26 | 70 | -1.13088 | -1.17181 | -1.17285 | -1.17299 |
| | V6Z-27 | 80 | -1.13089 | -1.17203 | -1.17270 | -1.17283 |
| | V6Z-28 | 80 | -1.13089 | -1.17203 | -1.17269 | -1.17283 |
| | V6Z-29 | 86 | -1.13089 | -1.17205 | -1.17266 | -1.17279 |
| | V6Z-30 | 86 | -1.13089 | -1.17205 | -1.17267 | -1.17280 |
| | V6Z-31 | 100 | -1.13090 | -1.17217 | -1.17257 | -1.17270 |
| | V6Z-[32-33] | 100 | -1.13090 | -1.17217 | -1.17268 | -1.17281 |
| | V6Z-[34-37] | 118 | -1.13090 | -1.17222 | -1.17266 | -1.17279 |
| | V6Z-[38-39] | 140 | -1.13090 | -1.17224 | -1.17261 | -1.17273 |
| | V6Z-[40-45] | 150 | -1.13090 | -1.17226 | -1.17256 | -1.17269 |
| | V6Z-[46-79] | 168 | -1.13090 | -1.17229 | -1.17254 | -1.17267 |

TABLE VI: [1/3] Ground-state energies (in Ha) of the LiH molecule calculated by HF, near-FCI (CIPSI+PT2), and self-consistent basis-set corrected near-FCI without and with the HF basis-set correction (denoted as SC(FCI+PBE) and SC(FCI+PBE)+ΔHF, respectively). VXZ-Y corresponds to the cc-pVXZ basis transformed to a basis of Y AO functions following the SABS building procedure. The notation VXZ-[$Y_n$-$Y_{n+a}$] means that the values are the same for the basis sets VXY-$Y_n$, VXY-$Y_{n+1}$, ..., VXY-$Y_{n+a-1}$, and VXY-$Y_{n+a}$. The FCI/CBS limit is -8.02482 Ha.

| LiH | Basis set | # active MOs | HF | FCI | SC(FCI+PBE) | SC(FCI+PBE)+ΔHF |
|---|---|---|---|---|---|---|
| | VDZ-[4-7] | 5 | -7.97539 | -7.99185 | -8.00469 | -8.01677 |
| | VDZ-8 | 9 | -7.98017 | -7.99894 | -8.00953 | -8.01683 |
| | VDZ-9 | 12 | -7.98147 | -8.00858 | -8.01321 | -8.01922 |
| | VDZ-10 | 13 | -7.98232 | -8.01002 | -8.01456 | -8.01972 |
| | VDZ-11 | 13 | -7.98232 | -8.01002 | -8.01460 | -8.01975 |
| | VDZ-12 | 18 | -7.98372 | -8.01437 | -8.01851 | -8.02226 |
| | VTZ-[4,5] | 5 | -7.97596 | -7.99267 | -8.00544 | -8.01696 |
| | VTZ-[6-8] | 8 | -7.98028 | -7.99634 | -8.00932 | -8.01652 |
| | VTZ-9 | 11 | -7.98340 | -7.99981 | -8.01260 | -8.01668 |
| | VTZ-10 | 12 | -7.98447 | -8.00140 | -8.01392 | -8.01693 |
| | VTZ-11 | 17 | -7.98509 | -8.00438 | -8.01549 | -8.01788 |
| | VTZ-12 | 20 | -7.98592 | -8.01781 | -8.02355 | -8.02510 |
| | VTZ-[13-15] | 21 | -7.98606 | -8.01837 | -8.02278 | -8.02420 |
| | VTZ-16 | 26 | -7.98627 | -8.01898 | -8.02319 | -8.02440 |
| | VTZ-[17,18] | 33 | -7.98643 | -8.01973 | -8.02368 | -8.02473 |
| | VTZ-19 | 38 | -7.98647 | -8.02061 | -8.02286 | -8.02386 |
| | VTZ-[20-23] | 41 | -7.98652 | -8.02151 | -8.02302 | -8.02397 |
| | VTZ-[24-41] | 42 | -7.98661 | -8.02212 | -8.02359 | -8.02446 |
| | VTZ-42 | 43 | -7.98664 | -8.02234 | -8.02378 | -8.02461 |
| | VQZ-[4,5] | 5 | -7.97603 | -7.99281 | -8.00557 | -8.01702 |
| | VQZ-[6-9] | 8 | -7.97985 | -7.99605 | -8.00895 | -8.01657 |
| | VQZ-[10,11] | 12 | -7.98304 | -8.00059 | -8.01089 | -8.01532 |
| | VQZ-12 | 15 | -7.98404 | -8.01500 | -8.02051 | -8.02394 |
| | VQZ-[13,14] | 16 | -7.98469 | -8.01585 | -8.02132 | -8.02411 |
| | VQZ-15 | 21 | -7.98561 | -8.01772 | -8.02277 | -8.02463 |
| | VQZ-16 | 22 | -7.98575 | -8.01817 | -8.02285 | -8.02458 |
| | VQZ-17 | 25 | -7.98651 | -8.01900 | -8.02364 | -8.02461 |
| | VQZ-18 | 30 | -7.98659 | -8.02043 | -8.02331 | -8.02419 |
| | VQZ-[19-21] | 35 | -7.98661 | -8.02065 | -8.02345 | -8.02432 |
| | VQZ-22 | 36 | -7.98696 | -8.02107 | -8.02385 | -8.02437 |
| | VQZ-23 | 39 | -7.98705 | -8.02276 | -8.02443 | -8.02485 |
| | VQZ-[24,25] | 44 | -7.98712 | -8.02288 | -8.02448 | -8.02483 |
| | VQZ-[26-28] | 51 | -7.98714 | -8.02316 | -8.02473 | -8.02507 |
| | VQZ-[29,30] | 58 | -7.98714 | -8.02326 | -8.02478 | -8.02511 |
| | VQZ-31 | 61 | -7.98715 | -8.02341 | -8.02455 | -8.02488 |
| | VQZ-32 | 62 | -7.98715 | -8.02350 | -8.02462 | -8.02494 |
| | VQZ-33 | 63 | -7.98716 | -8.02357 | -8.02468 | -8.02500 |
| | VQZ-34 | 72 | -7.98717 | -8.02366 | -8.02472 | -8.02503 |
| | VQZ-[35-38] | 79 | -7.98717 | -8.02381 | -8.02458 | -8.02489 |
| | VQZ-39 | 84 | -7.98717 | -8.02391 | -8.02453 | -8.02484 |

TABLE VII: [2/3] Ground-state energies (in Ha) of the LiH molecule calculated by HF, near-FCI (CIPSI+PT2), and self-consistent basis-set corrected near-FCI without and with the HF basis-set correction (denoted as SC(FCI+PBE) and SC(FCI+PBE)+ΔHF, respectively). VXZ-Y corresponds to the cc-pVXZ basis transformed to a basis of Y AO functions following the SABS building procedure. The notation VXZ-[$Y_n$-$Y_{n+a}$] means that the values are the same for the basis sets VXY-$Y_n$, VXY-$Y_{n+1}$, ..., VXY-$Y_{n+a-1}$, and VXY-$Y_{n+a}$. The FCI/CBS limit is -8.02482 Ha.

| LiH | Basis set | # active MOs | HF | FCI | SC(FCI+PBE) | SC(FCI+PBE)+ΔHF |
|---|---|---|---|---|---|---|
| | V5Z-[4-6] | 5 | -7.97604 | -7.99287 | -8.00561 | -8.01705 |
| | V5Z-[7,8] | 8 | -7.98198 | -7.99793 | -8.01108 | -8.01657 |
| | V5Z-9 | 11 | -7.98238 | -7.99900 | -8.01179 | -8.01689 |
| | V5Z-10 | 14 | -7.98326 | -8.01302 | -8.02133 | -8.02554 |
| | V5Z-[11,12] | 15 | -7.98391 | -8.01389 | -8.02195 | -8.02552 |
| | V5Z-13 | 16 | -7.98420 | -8.01421 | -8.02227 | -8.02555 |
| | V5Z-14 | 19 | -7.98543 | -8.01533 | -8.02336 | -8.02541 |
| | V5Z-15 | 20 | -7.98630 | -8.01710 | -8.02423 | -8.02541 |
| | V5Z-16 | 21 | -7.98651 | -8.01757 | -8.02375 | -8.02471 |
| | V5Z-17 | 22 | -7.98657 | -8.01778 | -8.02382 | -8.02472 |
| | V5Z-[18,19] | 27 | -7.98673 | -8.01954 | -8.02377 | -8.02452 |
| | V5Z-20 | 32 | -7.98673 | -8.01970 | -8.02385 | -8.02460 |
| | V5Z-[21,22] | 35 | -7.98683 | -8.02212 | -8.02454 | -8.02519 |
| | V5Z-23 | 38 | -7.98714 | -8.02247 | -8.02487 | -8.02520 |
| | V5Z-[24,25] | 39 | -7.98724 | -8.02298 | -8.02493 | -8.02517 |
| | V5Z-26 | 44 | -7.98724 | -8.02317 | -8.02506 | -8.02529 |
| | V5Z-[27-29] | 49 | -7.98728 | -8.02326 | -8.02510 | -8.02530 |
| | V5Z-[30-32] | 56 | -7.98728 | -8.02338 | -8.02517 | -8.02536 |
| | V5Z-33 | 60 | -7.98729 | -8.02362 | -8.02499 | -8.02517 |
| | V5Z-34 | 67 | -7.98730 | -8.02384 | -8.02484 | -8.02502 |
| | V5Z-35 | 68 | -7.98732 | -8.02387 | -8.02487 | -8.02503 |
| | V5Z-36 | 68 | -7.98732 | -8.02387 | -8.02485 | -8.02501 |
| | V5Z-[37-39] | 75 | -7.98732 | -8.02389 | -8.02487 | -8.02503 |
| | V5Z-40 | 78 | -7.98732 | -8.02390 | -8.02472 | -8.02488 |
| | V5Z-41 | 83 | -7.98732 | -8.02403 | -8.02465 | -8.02481 |
| | V5Z-42 | 90 | -7.98732 | -8.02412 | -8.02453 | -8.02469 |
| | V5Z-43 | 90 | -7.98732 | -8.02412 | -8.02455 | -8.02471 |
| | V5Z-44 | 90 | -7.98732 | -8.02412 | -8.02448 | -8.02464 |
| | V5Z-45 | 90 | -7.98732 | -8.02412 | -8.02452 | -8.02467 |
| | V5Z-46 | 90 | -7.98732 | -8.02408 | -8.02469 | -8.02484 |
| | V5Z-47 | 99 | -7.98732 | -8.02406 | -8.02466 | -8.02481 |
| | V5Z-48 | 99 | -7.98732 | -8.02413 | -8.02472 | -8.02488 |
| | V5Z-49 | 99 | -7.98732 | -8.02412 | -8.02472 | -8.02487 |
| | V5Z-50 | 99 | -7.98732 | -8.02413 | -8.02468 | -8.02483 |
| | V5Z-51 | 99 | -7.98732 | -8.02409 | -8.02470 | -8.02486 |
| | V5Z-52 | 106 | -7.98732 | -8.02415 | -8.02466 | -8.02482 |
| | V5Z-53 | 115 | -7.98732 | -8.02420 | -8.02443 | -8.02459 |
| | V5Z-54 | 115 | -7.98732 | -8.02420 | -8.02452 | -8.02468 |
| | V5Z-55 | 115 | -7.98732 | -8.02420 | -8.02452 | -8.02468 |
| | V5Z-56 | 120 | -7.98732 | -8.02427 | -8.02451 | -8.02466 |
| | V5Z-57 | 129 | -7.98732 | -8.02430 | -8.02445 | -8.02461 |
| | V5Z-58 | 129 | -7.98732 | -8.02430 | -8.02449 | -8.02464 |
| | V5Z-59 | 129 | -7.98732 | -8.02430 | -8.02450 | -8.02465 |
| | V5Z-60 | 129 | -7.98732 | -8.02430 | -8.02448 | -8.02464 |

TABLE VIII: [3/3] Ground-state energies (in Ha) of the LiH molecule calculated by HF, near-FCI (CIPSI+PT2), and self-consistent basis-set corrected near-FCI without and with the HF basis-set correction (denoted as SC(FCI+PBE) and SC(FCI+PBE)+ΔHF, respectively). VXZ-Y corresponds to the cc-pVXZ basis transformed to a basis of Y AO functions following the SABS building procedure. The notation VXZ-[$Y_n$-$Y_{n+a}$] means that the values are the same for the basis sets VXY-$Y_n$, VXY-$Y_{n+1}$, ..., VXY-$Y_{n+a-1}$, and VXY-$Y_{n+a}$. The FCI/CBS limit is -8.02482 Ha.

| LiH | Basis set | # active MOs | HF | FCI | SC(FCI+PBE) | SC(FCI+PBE)+ΔHF |
|---|---|---|---|---|---|---|
| | V5Z-61 | 129 | -7.98732 | -8.02430 | -8.02450 | -8.02466 |
| | V5Z-62 | 129 | -7.98732 | -8.02430 | -8.02454 | -8.02469 |
| | V5Z-63 | 140 | -7.98732 | -8.02432 | -8.02442 | -8.02458 |
| | V5Z-64 | 140 | -7.98732 | -8.02432 | -8.02446 | -8.02462 |
| | V5Z-65 | 140 | -7.98732 | -8.02432 | -8.02430 | -8.02445 |
| | V5Z-66 | 140 | -7.98732 | -8.02432 | -8.02449 | -8.02464 |
| | V5Z-67 | 140 | -7.98732 | -8.02432 | -8.02435 | -8.02451 |
| | V5Z-68 | 140 | -7.98732 | -8.02432 | -8.02447 | -8.02462 |
| | V5Z-69 | 140 | -7.98732 | -8.02432 | -8.02433 | -8.02449 |
| | V5Z-70 | 140 | -7.98732 | -8.02432 | -8.02425 | -8.02440 |
| | V5Z-71 | 140 | -7.98732 | -8.02432 | -8.02428 | -8.02443 |
| | V5Z-72 | 140 | -7.98732 | -8.02432 | -8.02437 | -8.02453 |
| | V5Z-73 | 140 | -7.98732 | -8.02432 | -8.02451 | -8.02467 |
| | V5Z-74 | 140 | -7.98732 | -8.02432 | -8.02432 | -8.02448 |
| | V5Z-75 | 140 | -7.98732 | -8.02432 | -8.02426 | -8.02441 |
| | V5Z-76 | 140 | -7.98732 | -8.02432 | -8.02440 | -8.02456 |
| | V5Z-77 | 140 | -7.98732 | -8.02432 | -8.02430 | -8.02445 |
| | V5Z-78 | 140 | -7.98732 | -8.02432 | -8.02428 | -8.02444 |
| | V5Z-79 | 140 | -7.98732 | -8.02432 | -8.02433 | -8.02449 |
| | V5Z-80 | 140 | -7.98732 | -8.02432 | -8.02431 | -8.02447 |
| | V5Z-81 | 145 | -7.98732 | -8.02431 | -8.02399 | -8.02415 |

TABLE IX: [1/2] Ground-state energies (in Ha) of the $H_2O$ molecule calculated by HF, near-FCI (CIPSI+PT2), and self-consistent basis-set corrected near-FCI without and with the HF basis-set correction (denoted as SC(FCI+PBE) and SC(FCI+PBE)+ΔHF, respectively). VXZ-Y corresponds to the cc-pVXZ basis transformed to a basis of Y AO functions following the SABS building procedure. The notation VXZ-[$Y_n$-$Y_{n+a}$] means that the values are the same for the basis sets VXY-$Y_n$, VXY-$Y_{n+1}$, ..., VXY-$Y_{n+a-1}$, and VXY-$Y_{n+a}$. The FCI/CBS limit is -76.37812 Ha.

| $H_2O$ | Basis set | # active MOs | HF | FCI | SC(FCI+PBE) | SC(FCI+PBE)+ΔHF |
|---|---|---|---|---|---|---|
| | VDZ-5 | 6 | -75.89241 | -75.93669 | -76.11929 | -76.29628 |
| | VDZ-6 | 7 | -75.90086 | -75.95934 | -76.13269 | -76.30124 |
| | VDZ-7 | 9 | -75.96623 | -76.02968 | -76.19811 | -76.30128 |
| | VDZ-8 | 9 | -75.96623 | -76.02968 | -76.19811 | -76.30128 |
| | VDZ-9 | 12 | -75.98044 | -76.11620 | -76.25492 | -76.34389 |
| | VDZ-10 | 12 | -75.98044 | -76.11620 | -76.25499 | -76.34396 |
| | VDZ-11 | 18 | -76.01858 | -76.17283 | -76.29347 | -76.34430 |
| | VDZ-12 | 18 | -76.01858 | -76.17283 | -76.29347 | -76.34430 |
| | VDZ-13 | 18 | -76.01858 | -76.17283 | -76.29347 | -76.34430 |
| | VDZ-14 | 18 | -76.01858 | -76.17283 | -76.29347 | -76.34430 |
| | VDZ-15 | 23 | -76.02677 | -76.24164 | -76.31537 | -76.35801 |
| | VTZ-5 | 6 | -75.90857 | -75.95344 | -76.13540 | -76.29623 |
| | VTZ-6 | 6 | -75.90857 | -75.95344 | -76.13540 | -76.29623 |
| | VTZ-7 | 8 | -75.97635 | -76.02689 | -76.20462 | -76.29768 |
| | VTZ-8 | 8 | -75.97635 | -76.02689 | -76.20461 | -76.29767 |
| | VTZ-9 | 11 | -75.99693 | -76.11476 | -76.26502 | -76.33749 |
| | VTZ-10 | 12 | -76.00181 | -76.13304 | -76.27671 | -76.34430 |
| | VTZ-11 | 12 | -76.00181 | -76.13304 | -76.27661 | -76.34420 |
| | VTZ-12 | 18 | -76.03306 | -76.17994 | -76.31259 | -76.34894 |
| | VTZ-13 | 20 | -76.03462 | -76.18539 | -76.31508 | -76.34987 |
| | VTZ-14 | 20 | -76.03462 | -76.18539 | -76.31508 | -76.34987 |
| | VTZ-15 | 20 | -76.03462 | -76.18539 | -76.31508 | -76.34987 |
| | VTZ-16 | 26 | -76.04399 | -76.20157 | -76.31989 | -76.34530 |
| | VTZ-17 | 31 | -76.05250 | -76.25599 | -76.34643 | -76.36333 |
| | VTZ-18 | 31 | -76.05250 | -76.25599 | -76.34643 | -76.36333 |
| | VTZ-19 | 36 | -76.05538 | -76.28894 | -76.34552 | -76.35954 |
| | VTZ-20 | 39 | -76.05554 | -76.30272 | -76.35240 | -76.36626 |
| | VTZ-21 | 39 | -76.05554 | -76.30298 | -76.35240 | -76.36626 |
| | VTZ-22 | 49 | -76.05664 | -76.31067 | -76.35578 | -76.36854 |
| | VTZ-23 | 56 | -76.05705 | -76.32636 | -76.36003 | -76.37239 |
| | VQZ-5 | 6 | -75.91275 | -75.95778 | -76.13974 | -76.29640 |
| | VQZ-6 | 6 | -75.91275 | -75.95778 | -76.13974 | -76.29640 |
| | VQZ-7 | 6 | -75.91275 | -75.95778 | -76.13974 | -76.29640 |
| | VQZ-8 | 8 | -75.97626 | -76.02635 | -76.20482 | -76.29796 |
| | VQZ-9 | 11 | -75.99855 | -76.11074 | -76.26425 | -76.33510 |
| | VQZ-10 | 12 | -76.00570 | -76.12947 | -76.27719 | -76.34089 |
| | VQZ-11 | 14 | -76.02138 | -76.14741 | -76.29062 | -76.33865 |
| | VQZ-12 | 14 | -76.02138 | -76.14741 | -76.29062 | -76.33865 |
| | VQZ-13 | 20 | -76.04618 | -76.19039 | -76.31636 | -76.33958 |
| | VQZ-14 | 20 | -76.04618 | -76.19039 | -76.31636 | -76.33958 |
| | VQZ-15 | 23 | -76.04840 | -76.21652 | -76.32652 | -76.34753 |
| | VQZ-16 | 28 | -76.05728 | -76.28404 | -76.34910 | -76.36123 |
| | VQZ-17 | 34 | -76.05950 | -76.29193 | -76.35589 | -76.36579 |
| | VQZ-18 | 39 | -76.06046 | -76.30063 | -76.36204 | -76.37098 |
| | VQZ-19 | 39 | -76.06046 | -76.30063 | -76.36205 | -76.37099 |
| | VQZ-20 | 39 | -76.06046 | -76.30065 | -76.36204 | -76.37098 |
| | VQZ-21 | 45 | -76.06207 | -76.30361 | -76.36256 | -76.36990 |
| | VQZ-22 | 45 | -76.06207 | -76.30361 | -76.36256 | -76.36990 |
| | VQZ-23 | 50 | -76.06247 | -76.31192 | -76.35916 | -76.36609 |

TABLE X: [2/2] Ground-state energies (in Ha) of the $H_2O$ molecule calculated by HF, near-FCI (CIPSI+PT2), and self-consistent basis-set corrected near-FCI without and with the HF basis-set correction (denoted as SC(FCI+PBE) and SC(FCI+PBE)+ΔHF, respectively). VXZ-Y corresponds to the cc-pVXZ basis transformed to a basis of Y AO functions following the SABS building procedure. The notation VXZ-[$Y_n$-$Y_{n+a}$] means that the values are the same for the basis sets VXY-$Y_n$, VXY-$Y_{n+1}$, ..., VXY-$Y_{n+a-1}$, and VXY-$Y_{n+a}$. The FCI/CBS limit is -76.37812 Ha.

| $H_2O$ | Basis set | # active MOs | HF | FCI | SC(FCI+PBE) | SC(FCI+PBE)+ΔHF |
|---|---|---|---|---|---|---|
| | V5Z-5 | 6 | -75.91383 | -75.95891 | -76.14081 | -76.29638 |
| | V5Z-6 | 6 | -75.91383 | -75.95891 | -76.14081 | -76.29638 |
| | V5Z-7 | 6 | -75.91383 | -75.95891 | -76.14081 | -76.29638 |
| | V5Z-8 | 8 | -75.99384 | -76.04603 | -76.22026 | -76.29583 |
| | V5Z-9 | 9 | -76.00422 | -76.07508 | -76.23959 | -76.30477 |
| | V5Z-10 | 12 | -76.01618 | -76.12626 | -76.27636 | -76.32958 |
| | V5Z-11 | 15 | -76.01756 | -76.15902 | -76.29319 | -76.34504 |
| | V5Z-12 | 15 | -76.01756 | -76.15902 | -76.29321 | -76.34506 |
| | V5Z-13 | 17 | -76.02137 | -76.16455 | -76.29813 | -76.34616 |
| | V5Z-14 | 23 | -76.05007 | -76.21406 | -76.33178 | -76.35112 |
| | V5Z-15 | 28 | -76.05818 | -76.27612 | -76.35656 | -76.36779 |
| | V5Z-16 | 28 | -76.05818 | -76.27612 | -76.35656 | -76.36779 |
| | V5Z-17 | 30 | -76.05939 | -76.27878 | -76.35751 | -76.36752 |
| | V5Z-18 | 30 | -76.05939 | -76.27878 | -76.35751 | -76.36752 |
| | V5Z-19 | 30 | -76.05939 | -76.27878 | -76.35751 | -76.36752 |
| | V5Z-20 | 30 | -76.05939 | -76.27878 | -76.35751 | -76.36752 |
| | V6Z-5 | 6 | -75.91390 | -75.95899 | -76.14088 | -76.29639 |
| | V6Z-6 | 6 | -75.91390 | -75.95899 | -76.14088 | -76.29639 |
| | V6Z-7 | 6 | -75.91390 | -75.95899 | -76.14088 | -76.29639 |
| | V6Z-8 | 8 | -75.99599 | -76.04790 | -76.22379 | -76.29720 |
| | V6Z-9 | 9 | -76.00502 | -76.07392 | -76.24098 | -76.30537 |
| | V6Z-10 | 12 | -76.01665 | -76.14766 | -76.29046 | -76.34322 |
| | V6Z-11 | 18 | -76.04304 | -76.19235 | -76.32124 | -76.34761 |
| | V6Z-12 | 18 | -76.04304 | -76.19233 | -76.32127 | -76.34763 |
| | V6Z-13 | 21 | -76.04482 | -76.19875 | -76.32480 | -76.34939 |
| | V6Z-14 | 22 | -76.04584 | -76.20378 | -76.32573 | -76.34930 |
| | V6Z-15 | 24 | -76.04619 | -76.20739 | -76.32728 | -76.35050 |
| | V6Z-16 | 24 | -76.04619 | -76.20740 | -76.32728 | -76.35050 |
| | V6Z-17 | 29 | -76.05504 | -76.26201 | -76.35272 | -76.36709 |
| | V6Z-18 | 32 | -76.05517 | -76.27309 | -76.35519 | -76.36943 |
| | V6Z-19 | 38 | -76.05960 | -76.28117 | -76.35808 | -76.36789 |
| | V6Z-20 | 38 | -76.05960 | -76.28166 | -76.35808 | -76.36789 |

TABLE XI: Ground-state energies (in Ha) of the $N_2$ molecule calculated by HF, near-FCI (CIPSI+PT2), and self-consistent basis-set corrected near-FCI without and with the HF basis-set correction (denoted as SC(FCI+PBE) and SC(FCI+PBE)+$\Delta$HF, respectively). VXZ-Y corresponds to the cc-pVXZ basis transformed to a basis of Y AO functions following the SABS building procedure. The notation VXZ-[$Y_n$-$Y_{n+a}$] means that the values are the same for the basis sets VXY-$Y_n$, VXY-$Y_{n+1}$, ..., VXY-$Y_{n+a-1}$, and VXY-$Y_{n+a}$. The FCI/CBS limit is -109.42498 Ha.

| $N_2$ | Basis set | # active MOs | HF | FCI | SC(FCI+PBE) | SC(FCI+PBE)+$\Delta$HF |
|---|---|---|---|---|---|---|
| | VQZ-10 | 14 | -108.82485 | -109.01533 | -109.20135 | -109.37101 |
| | VQZ-11 | 16 | -108.88278 | -109.10163 | -109.27284 | -109.38458 |
| | VQZ-[12-14] | 22 | -108.90058 | -109.14692 | -109.29652 | -109.39046 |
| | VQZ-[15-16] | 24 | -108.90226 | -109.15252 | -109.29290 | -109.38516 |
| | VQZ-[17-20] | 34 | -108.98089 | -109.31664 | -109.39284 | -109.40647 |
| | VQZ-[21-25] | 44 | -108.98341 | -109.32951 | -109.38867 | -109.39977 |
| | VQZ-26 | 58 | -108.98412 | -109.35139 | -109.39949 | -109.40989 |
| | VQZ-27 | 68 | -108.98955 | -109.36564 | -109.41443 | -109.41940 |
| | V5Z-10 | 14 | -108.80656 | -109.01099 | -109.18262 | -109.37057 |
| | V5Z-[11-13] | 16 | -108.89413 | -109.12739 | -109.28517 | -109.38556 |
| | V5Z-14 | 26 | -108.97053 | -109.28372 | -109.38187 | -109.40585 |
| | V5Z-[15-17] | 32 | -108.97450 | -109.29460 | -109.39378 | -109.41380 |
| | V5Z-18 | 34 | -108.97679 | -109.30157 | -109.39547 | -109.41320 |
| | V5Z-19 | 40 | -108.97763 | -109.31094 | -109.39763 | -109.41451 |

### D. Dissociation curves

TABLE XII: Ground-state energies (in Ha) used for the dissociation curves of $H_2$ at the HF, near-FCI (CIPSI+PT2), self-consistent basis-set corrected ADAPT-VQE without the HF basis-set correction (denoted as SC(A+PBE)), and with the HF basis-set correction (denoted as SC(A+PBE)+ΔHF). Distances are in Å. VXZ stands for the standard cc-pVXZ basis set.

| Basis set | Distance | HF | FCI | SC(A+PBE) | SC(A+PBE)+ΔHF |
|---|---|---|---|---|---|
| VDZ | 0.5 | -1.04880 | -1.07937 | -1.08802 | -1.10414 |
| | 0.6 | -1.10689 | -1.13917 | -1.14667 | -1.15616 |
| | 0.7 | -1.12692 | -1.16090 | -1.16748 | -1.17333 |
| | 0.8 | -1.12700 | -1.16275 | -1.16858 | -1.17246 |
| | 0.9 | -1.11639 | -1.15408 | -1.15930 | -1.16218 |
| | 1.0 | -1.10015 | -1.14007 | -1.14481 | -1.14724 |
| | 1.5 | -1.00219 | -1.06153 | -1.06513 | -1.06787 |
| | 2.0 | -0.92191 | -1.01759 | -1.02089 | -1.02522 |
| | 2.5 | -0.86533 | -1.00313 | -1.00631 | -1.01238 |
| | 3.0 | -0.82645 | -0.99955 | -1.00268 | -1.01043 |
| V5Z-8 | 0.5 | -1.05683 | -1.08907 | -1.09726 | -1.10535 |
| | 0.6 | -1.11193 | -1.14569 | -1.15284 | -1.15729 |
| | 0.7 | -1.13028 | -1.16548 | -1.17178 | -1.17428 |
| | 0.8 | -1.12938 | -1.16614 | -1.17170 | -1.17321 |
| | 0.9 | -1.11825 | -1.15679 | -1.16174 | -1.16276 |
| | 1.0 | -1.10177 | -1.14243 | -1.14689 | -1.14770 |
| | 1.5 | -1.00378 | -1.06363 | -1.06675 | -1.06791 |
| | 2.0 | -0.92434 | -1.01944 | -1.02219 | -1.02409 |
| | 2.5 | -0.86969 | -1.00467 | -1.00739 | -1.00911 |
| | 3.0 | -0.83308 | -1.00100 | -1.00373 | -1.00484 |
| VTZ | 0.5 | - | -1.10087 | - | - |
| | 0.6 | - | -1.15352 | - | - |
| | 0.7 | - | -1.17101 | - | - |
| | 0.8 | - | -1.17041 | - | - |
| | 0.9 | - | -1.16041 | - | - |
| | 1.0 | - | -1.14576 | - | - |
| | 1.5 | - | -1.06617 | - | - |
| | 2.0 | - | -1.02046 | - | - |
| | 2.5 | - | -1.00467 | - | - |
| | 3.0 | - | -1.00072 | - | - |
| V5Z | 0.5 | -1.06492 | -1.10397 | - | - |
| | 0.6 | -1.11638 | -1.15581 | - | - |
| | 0.7 | -1.13278 | -1.17297 | - | - |
| | 0.8 | -1.13089 | -1.17223 | - | - |
| | 0.9 | -1.11927 | -1.16216 | - | - |
| | 1.0 | -1.10258 | -1.14748 | - | - |
| | 1.5 | -1.00493 | -1.06795 | - | - |
| | 2.0 | -0.92624 | -1.02186 | - | - |
| | 2.5 | -0.87140 | -1.00550 | - | - |
| | 3.0 | -0.83420 | -1.00124 | - | - |

TABLE XIII: Ground-state energies (in Ha) used for the dissociation curves of LiH at the HF, near-FCI (CIPSI+PT2), self-consistent basis-set corrected ADAPT-VQE without the HF basis-set correction (denoted as SC(A+PBE)), and with the HF basis-set correction (denoted as SC(A+PBE)+ΔHF). Distances are in Å. VXZ stands for the standard cc-pVXZ basis set.

| Basis set | Distance | HF | FCI | SC(A+PBE) | SC(A+PBE)+ΔHF |
|---|---|---|---|---|---|
| 6-31G | 0.5 | -7.14721 | -7.16953 | -7.17775 | -7.23149 |
| | 0.75 | -7.66281 | -7.68441 | -7.69458 | -7.72292 |
| | 1.0 | -7.87136 | -7.89039 | -7.90091 | -7.91794 |
| | 1.25 | -7.95144 | -7.96925 | -7.97975 | -7.99182 |
| | 1.5 | -7.97686 | -7.99510 | -8.00533 | -8.01428 |
| | 1.75 | -7.97824 | -7.99809 | -8.00780 | -8.01473 |
| | 2.0 | -7.96887 | -7.99121 | -8.00025 | -8.00617 |
| | 2.25 | -7.95492 | -7.98053 | -7.98884 | -7.99461 |
| | 2.5 | -7.93936 | -7.96907 | -7.97663 | -7.98291 |
| | 2.75 | -7.92365 | -7.95844 | -7.96522 | -7.97253 |
| | 3.0 | -7.90850 | -7.94951 | -7.95550 | -7.96420 |
| V5Z-7 | 0.5 | -7.10996 | -7.13045 | -7.14080 | -7.23179 |
| | 0.75 | -7.65310 | -7.66747 | -7.68139 | -7.71943 |
| | 1.0 | -7.87189 | -7.88480 | -7.89919 | -7.91570 |
| | 1.25 | -7.95443 | -7.96789 | -7.98184 | -7.99092 |
| | 1.5 | -7.97979 | -7.99488 | -8.00827 | -8.01429 |
| | 1.75 | -7.98055 | -7.99819 | -8.01091 | -8.01554 |
| | 2.0 | -7.97042 | -7.99152 | -8.00347 | -8.00784 |
| | 2.25 | -7.95565 | -7.98110 | -7.99226 | -7.99729 |
| | 2.5 | -7.93924 | -7.97003 | -7.98041 | -7.98681 |
| | 2.75 | -7.92265 | -7.95988 | -7.96953 | -7.97783 |
| | 3.0 | -7.90660 | -7.95145 | -7.96043 | -7.97104 |
| VDZ | 0.5 | - | -7.19664 | - | - |
| | 0.75 | - | -7.71273 | - | - |
| | 1.0 | - | -7.91535 | - | - |
| | 1.25 | - | -7.99037 | - | - |
| | 1.5 | - | -8.01264 | - | - |
| | 1.75 | - | -8.01278 | - | - |
| | 2.0 | - | -8.00361 | - | - |
| | 2.25 | - | -7.99108 | - | - |
| | 2.5 | - | -7.97809 | - | - |
| | 2.75 | - | -7.96613 | - | - |
| | 3.0 | - | -7.95594 | - | - |
| V5Z | 0.5 | -7.20095 | -7.24405 | - | - |
| | 0.75 | -7.69115 | -7.73130 | - | - |
| | 1.0 | -7.88839 | -7.92707 | - | - |
| | 1.25 | -7.96350 | -8.00106 | - | - |
| | 1.5 | -7.98581 | -8.02285 | - | - |
| | 1.75 | -7.98517 | -8.02236 | - | - |
| | 2.0 | -7.97479 | -8.01280 | - | - |
| | 2.25 | -7.96068 | -8.00003 | - | - |
| | 2.5 | -7.94564 | -7.98672 | - | - |
| | 2.75 | -7.93096 | -7.97443 | - | - |
| | 3.0 | -7.91720 | -7.96344 | - | - |

TABLE XIV: Ground-state energies (in Ha) used for the dissociation curves of $N_2$ at the HF, near-FCI (CIPSI+PT2), self-consistent basis-set corrected ADAPT-VQE without the HF basis-set correction (denoted as SC(A+PBE)), and with the HF basis-set correction (denoted as SC(A+PBE)+ΔHF). Distances are in Å. VXZ stands for the standard cc-pVXZ basis set.

| Basis set | Distance | HF | FCI | SC(A+PBE) | SC(A+PBE)+ΔHF |
|---|---|---|---|---|---|
| STO-3G | 0.8 | -106.68080 | -106.76594 | -106.99161 | -108.82882 |
| | 0.9 | -107.18719 | -107.29271 | -107.51568 | -109.18175 |
| | 1.0977 | -107.49589 | -107.65251 | -107.86975 | -109.36662 |
| | 1.2 | -107.48778 | -107.67707 | -107.88963 | -109.35016 |
| | 1.5 | -107.27245 | -107.58147 | -107.78293 | -109.22200 |
| | 2.0 | -106.87150 | -107.45512 | -107.65901 | -109.15567 |
| | 2.5 | -106.61696 | -107.44041 | -107.63628 | -109.18056 |
| V5Z-6 | 0.8 | -107.89375 | -107.97171 | -108.19082 | -108.81508 |
| | 0.9 | -108.39476 | -108.49175 | -108.70783 | -109.16634 |
| | 1.0977 | -108.74519 | -108.88869 | -109.09851 | -109.34608 |
| | 1.2 | -108.76756 | -108.93985 | -109.14120 | -109.32195 |
| | 1.5 | -108.63207 | -108.90483 | -109.09718 | -109.17662 |
| | 2 | -108.32055 | -108.81060 | -109.00808 | -109.05568 |
| | 2.5 | -108.10572 | -108.80176 | -109.00012 | -109.05564 |
| VDZ | 0.8 | - | -108.66035 | - | - |
| | 0.9 | - | -109.05746 | - | - |
| | 1.1 | - | -109.27657 | - | - |
| | 1.2 | - | -109.26410 | - | - |
| | 1.5 | - | -109.12459 | - | - |
| | 2.0 | - | -108.98115 | - | - |
| | 2.5 | - | -108.95868 | - | - |
| VTZ | 0.8 | - | -108.82771 | - | - |
| | 0.9 | - | -109.18511 | - | - |
| | 1.1 | - | -109.36884 | - | - |
| | 1.2 | - | -109.34807 | - | - |
| | 1.5 | - | -109.20218 | - | - |
| | 2.0 | - | -109.04838 | - | - |
| | 2.5 | - | -109.01953 | - | - |
| V5Z | 0.8 | -108.51801 | - | - | - |
| | 0.9 | -108.85326 | - | - | - |
| | 1.0977 | -108.99276 | - | - | - |
| | 1.2 | -108.94831 | - | - | - |
| | 1.5 | -108.71151 | - | - | - |
| | 2.0 | -108.36816 | - | - | - |
| | 2.5 | -108.16125 | - | - | - |

### E. Dipole moments

TABLE XV: Dipole moments (in atomic units) of LiH and $H_2O$ computed as expectation values of HF and near-FCI (CIPSI) wave functions, and the near-FCI dipole moments with the HF basis-set correction $\Delta\text{HF} = d_{\text{HF}}^{\text{aug-cc-pV5Z}} - d_{\text{HF}}^{\mathcal{B}}$, where $d_{\text{HF}}^{\text{aug-cc-pV5Z}}$ is the aug-cc-pV5Z HF dipole moment and $d_{\text{HF}}^{\mathcal{B}}$ is the HF dipole moment in the basis set $\mathcal{B}$ considered. aug-cc-pVXZ values are provided for informational purposes.

| LiH | $N_{\text{qubits}}$ | HF | FCI | FCI + ΔHF |
|---|---|---|---|---|
| STO-3G | 10 | -1.91107 | -1.81835 | -2.26857 |
| pcseg-0 | 14 | -2.47768 | -2.33313 | -2.21674 |
| 6-31G | 20 | -2.33223 | -2.16646 | -2.19552 |
| V5Z-4 | 10 | -2.57388 | -2.37818 | -2.16559 |
| V5Z-7 | 16 | -2.38299 | -2.23095 | -2.20925 |
| V5Z-10 | 28 | -2.32149 | -2.24997 | -2.28977 |
| cc-pVDZ | 36 | -2.33994 | -2.25566 | -2.27701 |
| cc-pVTZ | 86 | -2.35488 | -2.29998 | -2.30639 |
| cc-pVQZ | 190 | -2.35762 | -2.30361 | -2.30728 |
| cc-pV5Z | 290 | -2.36017 | -2.30647 | -2.30759 |
| aug-cc-pVDZ | 62 | -2.37055 | -2.32496 | -2.3157 |
| aug-cc-pVTZ | 136 | -2.36235 | -2.31028 | -2.30922 |
| aug-cc-pVQZ | 250 | -2.36152 | -2.30792 | -2.30769 |
| aug-cc-pV5Z | 412 | -2.36129 | -2.30787 | -2.30787 |
| $H_2O$ | $N_{\text{qubits}}$ | HF | FCI | FCI + ΔHF |
| STO-3G | 12 | -0.67878 | -0.63584 | -0.73662 |
| pcseg-0 | 24 | -1.00341 | -0.95822 | -0.73437 |
| 6-31G | 24 | -1.03512 | -0.9902 | -0.73464 |
| V5Z-10 | 24 | -1.02208 | -0.99305 | -0.75053 |
| V5Z-11 | 30 | -1.02389 | -0.99185 | -0.74752 |
| cc-pVDZ | 46 | -0.80943 | -0.76073 | -0.73086 |
| cc-pVTZ | 114 | -0.79709 | -0.74858 | -0.73105 |
| cc-pVQZ | 228 | -0.79006 | -0.74409 | -0.73359 |
| cc-pV5Z | 400 | -0.78783 | -0.74241 | -0.73414 |
| aug-cc-pVDZ | 80 | -0.78671 | -0.72703[a] | -0.71988[a] |
| aug-cc-pVTZ | 181 | -0.78038 | -0.72364[a] | -0.72282[a] |
| aug-cc-pVQZ | 342 | -0.77955 | -0.72695[a] | -0.72696[a] |
| aug-cc-pV5Z | 572 | -0.77956 | -0.72815[a] | -0.72815[a] |

[a] CCSD(T) values from Ref. [13].

## III. SABS

In this section, we give the basis functions in our SABS used in Table II of the paper.

### A. $H_2$, SABS/V5Z-8

```
HYDROGEN
S 8
               1  4.02E+02   2.79E-04
               2  6.02E+01   2.17E-03
               3  1.37E+01   1.12E-02
               4  3.91E+00   4.49E-02
               5  1.28E+00   1.42E-01
               6   4.66E-01   3.31E-01
               7   1.81E-01   4.36E-01
               8   7.28E-02   1.76E-01
S 1
               1   1.81E-01  1.00E+00
S 1
               1   7.28E-02  1.00E+00
P 1
               1   6.49E-01  1.00E+00
```

## B. LiH, SABS/V5Z-4

```
LITHIUM
S 14
   1  2.949300E+04  1.800000E-05
   2  4.417101E+03  1.410000E-04
   3  1.005223E+03  7.390000E-04
   4  2.847009E+02  3.107000E-03
   5  9.286543E+01  1.113500E-02
   6  3.351179E+01  3.467000E-02
   7  1.304180E+01  9.217100E-02
   8  5.357536E+00  1.995760E-01
   9  2.279338E+00  3.288360E-01
  10  9.939900E-01  3.459750E-01
  11  4.334710E-01  1.427610E-01
  12  9.556600E-02  5.319000E-03
  13  4.465700E-02  -2.101000E-03
  14  2.063300E-02  8.150000E-04
S 14
   1  2.949300E+04  -3.000000E-06
   2  4.417101E+03  -2.200000E-05
   3  1.005223E+03  -1.150000E-04
   4  2.847009E+02  -4.870000E-04
   5  9.286543E+01  -1.746000E-03
   6  3.351179E+01  -5.520000E-03
   7  1.304180E+01  -1.492800E-02
   8  5.357536E+00  -3.420600E-02
   9  2.279338E+00  -6.215500E-02
  10  9.939900E-01  -9.590200E-02
  11  4.334710E-01  -1.039720E-01
  12  9.556600E-02  3.071510E-01
  13  4.465700E-02  5.790280E-01
  14  2.063300E-02  2.232310E-01
P 8
   1  1.966350E+01  5.400000E-04
   2  4.623110E+00  3.865000E-03
   3  1.413780E+00  1.517100E-02
   4  4.737210E-01  4.920400E-02
   5  1.761510E-01  1.546610E-01
   6  7.267500E-02  3.600950E-01
   7  3.214100E-02  4.418520E-01
   8  1.455600E-02  1.560000E-01
HYDROGEN
S 8
   1  4.020000E+02  2.790000E-04
   2  6.024000E+01  2.165000E-03
   3  1.373000E+01  1.120100E-02
   4  3.905000E+00  4.487800E-02
   5  1.283000E+00  1.422990E-01
   6  4.655000E-01  3.309790E-01
   7  1.811000E-01  4.362690E-01
   8  7.279000E-02  1.764400E-01
```

### C. LiH, SABS/V5Z-7

```
LITHIUM
S 14
  1  2.949300E+04  1.800000E-05
  2  4.417101E+03  1.410000E-04
  3  1.005223E+03  7.390000E-04
  4  2.847009E+02  3.107000E-03
  5  9.286543E+01  1.113500E-02
  6  3.351179E+01  3.467000E-02
  7  1.304180E+01  9.217100E-02
  8  5.357536E+00  1.995760E-01
  9  2.279338E+00  3.288360E-01
 10  9.939900E-01  3.459750E-01
 11  4.334710E-01  1.427610E-01
 12  9.556600E-02  5.319000E-03
 13  4.465700E-02  -2.101000E-03
 14  2.063300E-02  8.150000E-04
S 14
  1  2.949300E+04  -3.000000E-06
  2  4.417101E+03  -2.200000E-05
  3  1.005223E+03  -1.150000E-04
  4  2.847009E+02  -4.870000E-04
  5  9.286543E+01  -1.746000E-03
  6  3.351179E+01  -5.520000E-03
  7  1.304180E+01  -1.492800E-02
  8  5.357536E+00  -3.420600E-02
  9  2.279338E+00  -6.215500E-02
 10  9.939900E-01  -9.590200E-02
 11  4.334710E-01  -1.039720E-01
 12  9.556600E-02  3.071510E-01
 13  4.465700E-02  5.790280E-01
 14  2.063300E-02  2.232310E-01
P 8
  1  1.966350E+01  5.400000E-04
  2  4.623110E+00  3.865000E-03
  3  1.413780E+00  1.517100E-02
  4  4.737210E-01  4.920400E-02
  5  1.761510E-01  1.546610E-01
  6  7.267500E-02  3.600950E-01
  7  3.214100E-02  4.418520E-01
  8  1.455600E-02  1.560000E-01
P 1
  1  3.214100E-02  1.000000E+00
HYDROGEN
S 8
  1  4.020000E+02  2.790000E-04
  2  6.024000E+01  2.165000E-03
  3  1.373000E+01  1.120100E-02
  4  3.905000E+00  4.487800E-02
  5  1.283000E+00  1.422990E-01
  6  4.655000E-01  3.309790E-01
  7  1.811000E-01  4.362690E-01
  8  7.279000E-02  1.764400E-01
```

### D. LiH, SABS/V5Z-10

LITHIUM

S 14

| | | |
|---|---|---|
| 1 | 2.95E+04 | 1.80E-05 |
| 2 | 4.42E+03 | 1.41E-04 |
| 3 | 1.01E+03 | 7.39E-04 |
| 4 | 2.85E+02 | 3.11E-03 |
| 5 | 9.29E+01 | 1.11E-02 |
| 6 | 3.35E+01 | 3.47E-02 |
| 7 | 1.30E+01 | 9.22E-02 |
| 8 | 5.36E+00 | 2.00E-01 |
| 9 | 2.28E+00 | 3.29E-01 |
| 10 | 9.94E-01 | 3.46E-01 |
| 11 | 4.33E-01 | 1.43E-01 |
| 12 | 9.56E-02 | 5.32E-03 |
| 13 | 4.47E-02 | -2.10E-03 |
| 14 | 2.06E-02 | 8.15E-04 |

S 14

| | | |
|---|---|---|
| 1 | 2.95E+04 | -3.00E-06 |
| 2 | 4.42E+03 | -2.20E-05 |
| 3 | 1.01E+03 | -1.15E-04 |
| 4 | 2.85E+02 | -4.87E-04 |
| 5 | 9.29E+01 | -1.75E-03 |
| 6 | 3.35E+01 | -5.52E-03 |
| 7 | 1.30E+01 | -1.49E-02 |
| 8 | 5.36E+00 | -3.42E-02 |
| 9 | 2.28E+00 | -6.22E-02 |
| 10 | 9.94E-01 | -9.59E-02 |
| 11 | 4.33E-01 | -1.04E-01 |
| 12 | 9.56E-02 | 3.07E-01 |
| 13 | 4.47E-02 | 5.79E-01 |
| 14 | 2.06E-02 | 2.23E-01 |

P 1

| | | |
|---|---|---|
| 1 | 7.27E-02 | 1.00E+00 |

P 8

| | | |
|---|---|---|
| 1 | 1.97E+01 | 5.40E-04 |
| 2 | 4.62E+00 | 3.87E-03 |
| 3 | 1.41E+00 | 1.52E-02 |
| 4 | 4.74E-01 | 4.92E-02 |
| 5 | 1.76E-01 | 1.55E-01 |
| 6 | 7.27E-02 | 3.60E-01 |
| 7 | 3.21E-02 | 4.42E-01 |
| 8 | 1.46E-02 | 1.56E-01 |

P 1

| | | |
|---|---|---|
| 1 | 3.21E-02 | 1.00E+00 |

HYDROGEN

S 8

| | | |
|---|---|---|
| 1 | 4.02E+02 | 2.79E-04 |
| 2 | 6.02E+01 | 2.17E-03 |
| 3 | 1.37E+01 | 1.12E-02 |
| 4 | 3.91E+00 | 4.49E-02 |
| 5 | 1.28E+00 | 1.42E-01 |
| 6 | 4.66E-01 | 3.31E-01 |
| 7 | 1.81E-01 | 4.36E-01 |
| 8 | 7.28E-02 | 1.76E-01 |

P 1

| | | |
|---|---|---|
| 1 | 2.46E-01 | 1.00E+00 |

## E. $H_2O$, SABS/V5Z-10

```
OXYGEN
S 14
    1 1.642000E+05  2.600000E-05
    2 2.459000E+04  2.050000E-04
    3 5.592000E+03  1.076000E-03
    4 1.582000E+03  4.522000E-03
    5 5.161000E+02  1.610800E-02
    6 1.872000E+02  4.908500E-02
    7 7.393000E+01  1.248570E-01
    8 3.122000E+01  2.516860E-01
    9 1.381000E+01  3.624200E-01
   10 6.256000E+00  2.790510E-01
   11 2.776000E+00  6.355200E-02
   12 1.138000E+00  1.063000E-03
   13 4.600000E-01  1.144000E-03
   14 1.829000E-01  -4.000000E-05
S 14
    1 1.642000E+05  -6.000000E-06
    2 2.459000E+04  -4.600000E-05
    3 5.592000E+03  -2.440000E-04
    4 1.582000E+03  -1.031000E-03
    5 5.161000E+02  -3.688000E-03
    6 1.872000E+02  -1.151400E-02
    7 7.393000E+01  -3.043500E-02
    8 3.122000E+01  -6.814700E-02
    9 1.381000E+01  -1.203680E-01
   10 6.256000E+00  -1.482600E-01
   11 2.776000E+00  9.905000E-03
   12 1.138000E+00  3.842860E-01
   13 4.600000E-01  5.368050E-01
   14 1.829000E-01  2.026870E-01
S 1
    1 1.829000E-01  1.000000E+00
P 8
    1 1.955000E+02  9.180000E-04
    2 4.616000E+01  7.388000E-03
    3 1.458000E+01  3.495800E-02
    4 5.296000E+00  1.154310E-01
    5 2.094000E+00  2.568030E-01
    6 8.471000E-01  3.739380E-01
    7 3.368000E-01  3.434470E-01
    8 1.285000E-01  1.297060E-01
P 1
    1 1.285000E-01  1.000000E+00
HYDROGEN
S 8
    1 4.020000E+02  2.790000E-04
    2 6.024000E+01  2.165000E-03
    3 1.373000E+01  1.120100E-02
    4 3.905000E+00  4.487800E-02
    5 1.283000E+00  1.422990E-01
    6 4.655000E-01  3.309790E-01
    7 1.811000E-01  4.362690E-01
    8 7.279000E-02  1.764400E-01
S 1
    1 1.811000E-01  1.000000E+00
```

### F. $N_2$, SABS/V5Z-6

NITROGEN
S 14

| | | |
|---|---|---|
| 1 | 1.292000E+05 | 2.500000E-05 |
| 2 | 1.935000E+04 | 1.970000E-04 |
| 3 | 4.404000E+03 | 1.032000E-03 |
| 4 | 1.248000E+03 | 4.325000E-03 |
| 5 | 4.080000E+02 | 1.538000E-02 |
| 6 | 1.482000E+02 | 4.686700E-02 |
| 7 | 5.850000E+01 | 1.201160E-01 |
| 8 | 2.459000E+01 | 2.456950E-01 |
| 9 | 1.081000E+01 | 3.613790E-01 |
| 10 | 4.882000E+00 | 2.872830E-01 |
| 11 | 2.195000E+00 | 7.017100E-02 |
| 12 | 8.715000E-01 | 1.831000E-03 |
| 13 | 3.504000E-01 | 8.350000E-04 |
| 14 | 1.397000E-01 | -6.000000E-06 |

S 14

| | | |
|---|---|---|
| 1 | 1.292000E+05 | -6.000000E-06 |
| 2 | 1.935000E+04 | -4.300000E-05 |
| 3 | 4.404000E+03 | -2.270000E-04 |
| 4 | 1.248000E+03 | -9.580000E-04 |
| 5 | 4.080000E+02 | -3.416000E-03 |
| 6 | 1.482000E+02 | -1.066700E-02 |
| 7 | 5.850000E+01 | -2.827900E-02 |
| 8 | 2.459000E+01 | -6.402000E-02 |
| 9 | 1.081000E+01 | -1.139320E-01 |
| 10 | 4.882000E+00 | -1.469950E-01 |
| 11 | 2.195000E+00 | -7.251000E-03 |
| 12 | 8.715000E-01 | 3.661830E-01 |
| 13 | 3.504000E-01 | 5.479080E-01 |
| 14 | 1.397000E-01 | 2.166450E-01 |

P 8

| | | |
|---|---|---|
| 1 | 1.470000E+02 | 8.920000E-04 |
| 2 | 3.476000E+01 | 7.082000E-03 |
| 3 | 1.100000E+01 | 3.281600E-02 |
| 4 | 3.995000E+00 | 1.082090E-01 |
| 5 | 1.587000E+00 | 2.480940E-01 |
| 6 | 6.533000E-01 | 3.745130E-01 |
| 7 | 2.686000E-01 | 3.484140E-01 |
| 8 | 1.067000E-01 | 1.283400E-01 |

## IV. ADAPT-VQE ENERGY CONVERGENCE

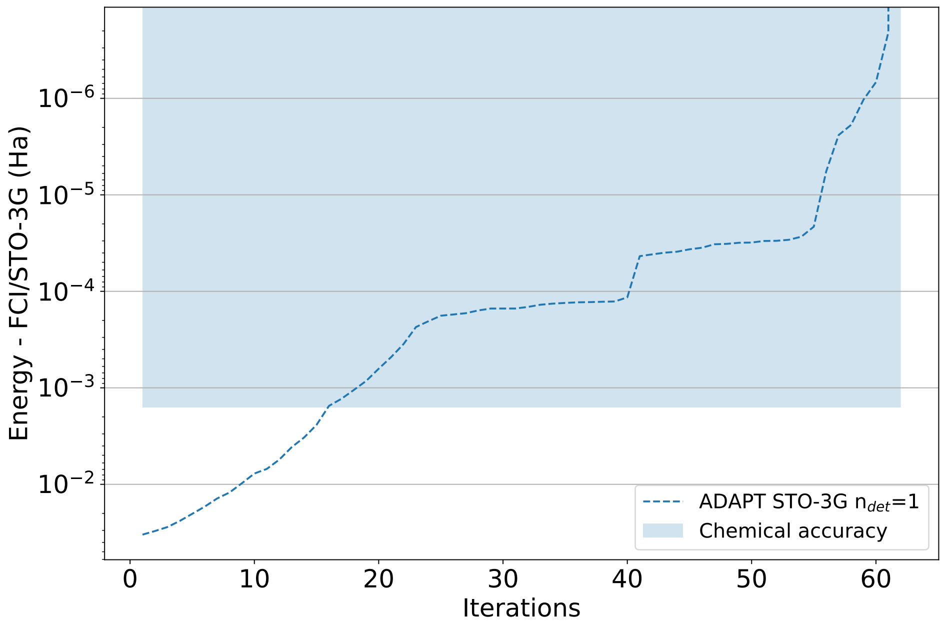


FIG. 1: Error in the ADAPT-VQE energy with respect to the FCI energy with the number of VQE iterations for the $H_2O$ molecule with the STO-3G basis set. The starting point is the HF determinant. The number of required qubits is 12.

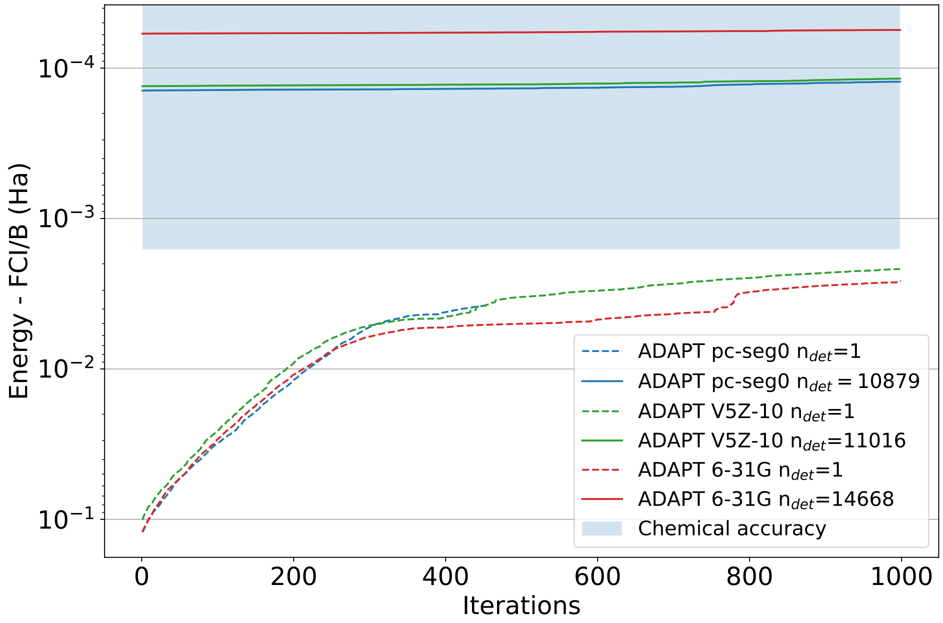


FIG. 2: Error in the ADAPT-VQE energy with respect to the FCI energy with the number of VQE iterations for the $H_2O$ molecule with the pcseg-0, SABS/V5Z-10, and 6-31G basis sets. The quantity $n_{\rm det}$ corresponds to the the number of determinants used for the initial state. For $n_{\rm det} = 1$, the initial state is the HF determinant. For the other cases, we use the CIPSI method to select the determinants. The number of required qubits is 24.

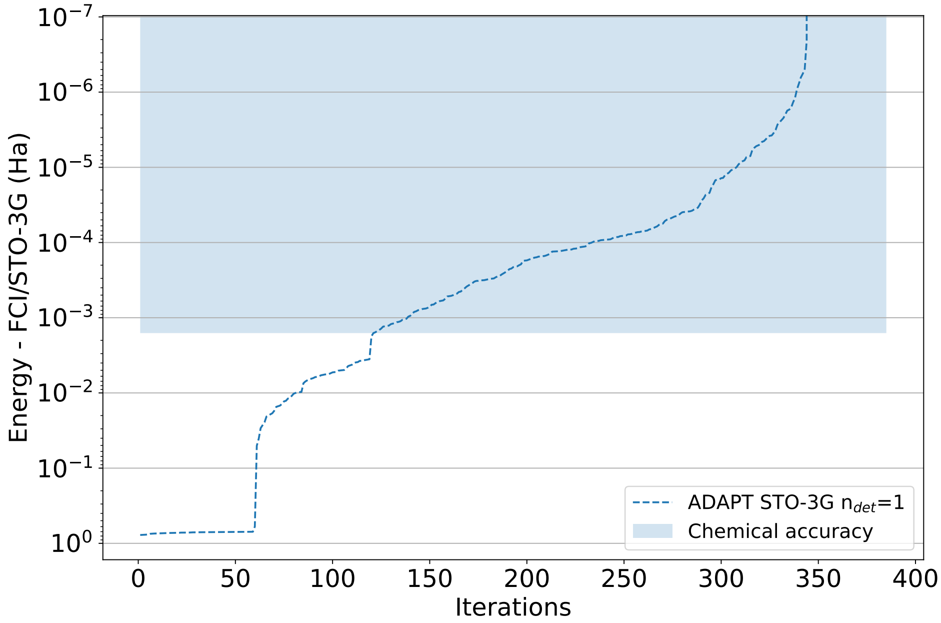


FIG. 3: Error in the ADAPT-VQE energy with respect to the FCI energy with the number of VQE iterations for the $N_2$ molecule with the STO-3G basis set. The starting point is the HF determinant. The number of required qubits is 16.

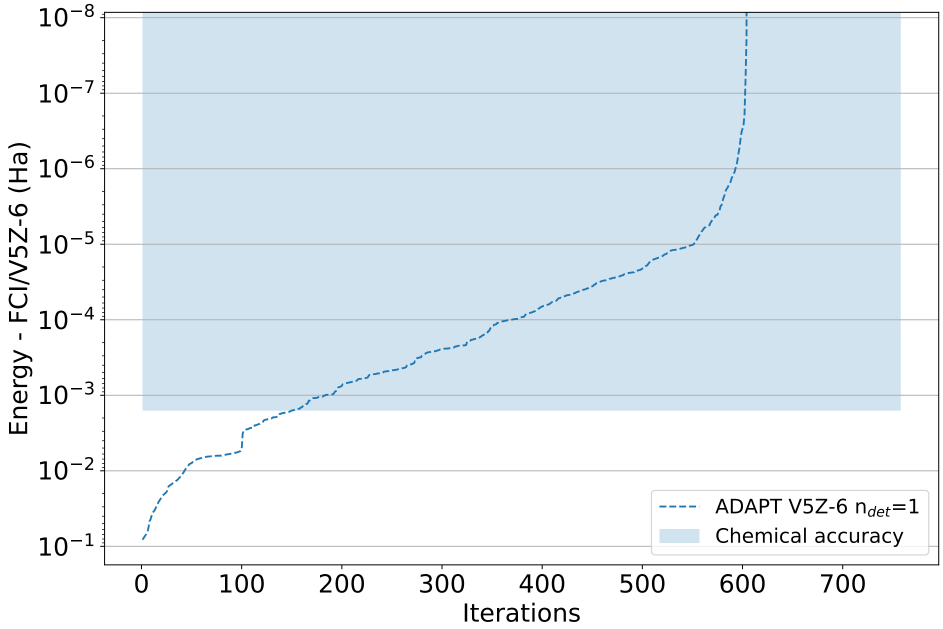


FIG. 4: Error in the ADAPT-VQE energy with respect to the FCI energy with the number of VQE iterations for the $N_2$ molecule with the SABS/V5Z-6 basis. The starting point is the HF determinant. The number of required qubits is 16.

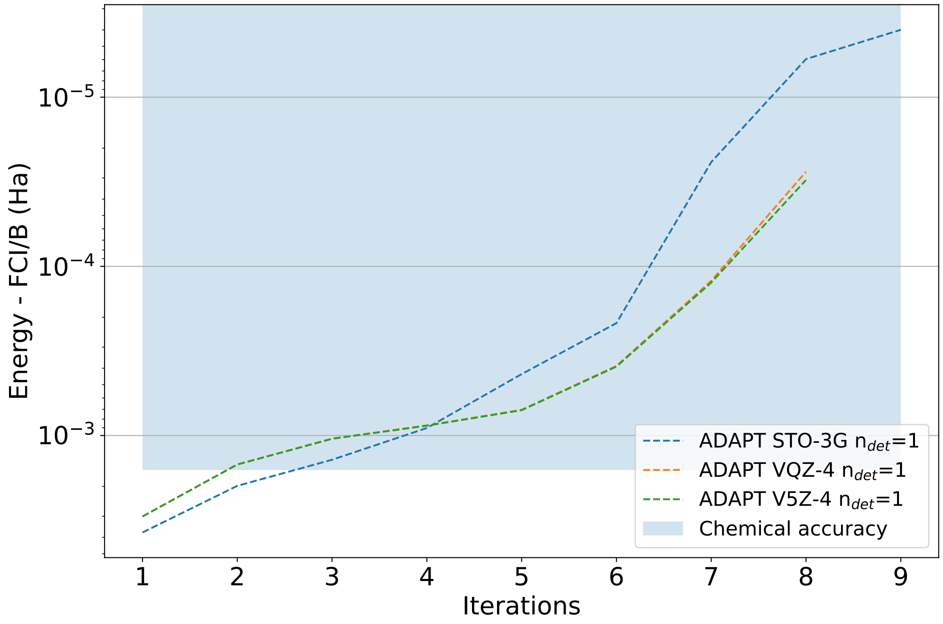


FIG. 5: Error in the ADAPT-VQE energy with respect to the FCI energy with the number of VQE iterations for the LiH molecule with the STO-3G, SABS/VQZ-4, and SABS/V5Z-4 basis sets. The starting point is the HF determinant. The number of required qubits is 10.

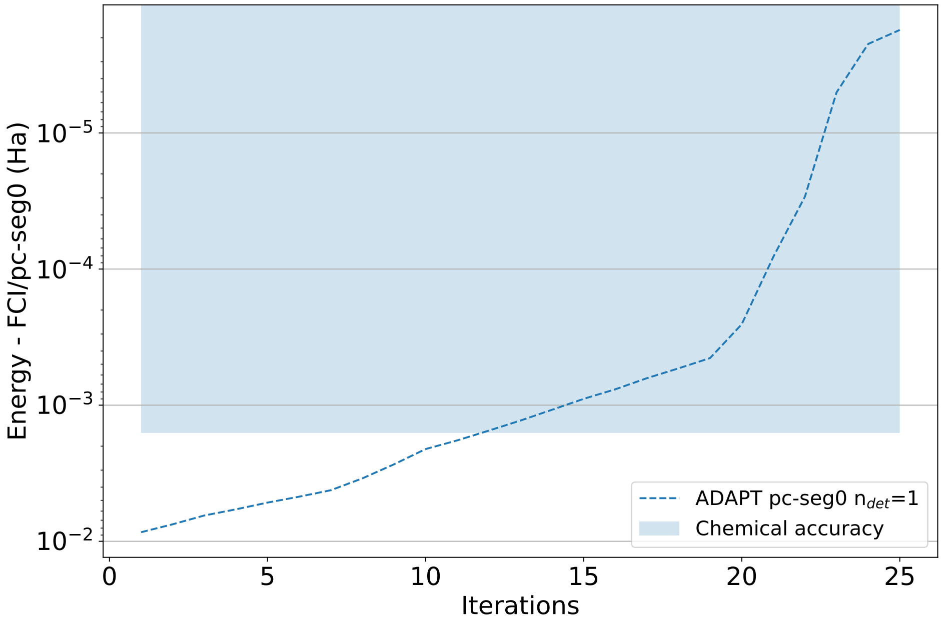


FIG. 6: Error in the ADAPT-VQE energy with respect to the FCI energy with the number of VQE iterations for the LiH molecule with the pcseg-0 basis. The starting point is the HF determinant. The number of required qubits is 14.

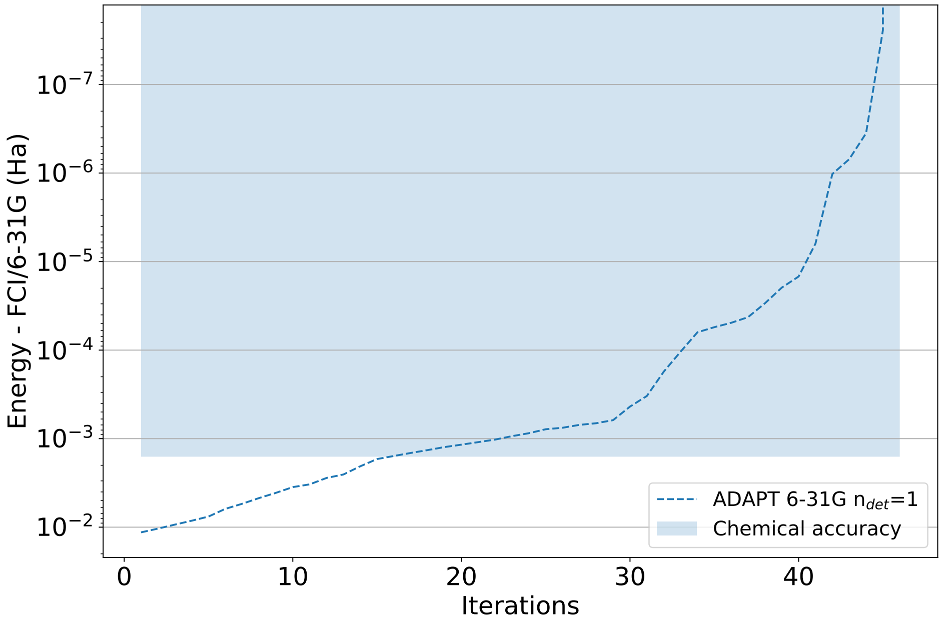


FIG. 7: Error in the ADAPT-VQE energy with respect to the FCI energy with the number of VQE iterations for the LiH molecule with the 6-31G basis set. The starting point is the HF determinant. The number of required qubits is 20.

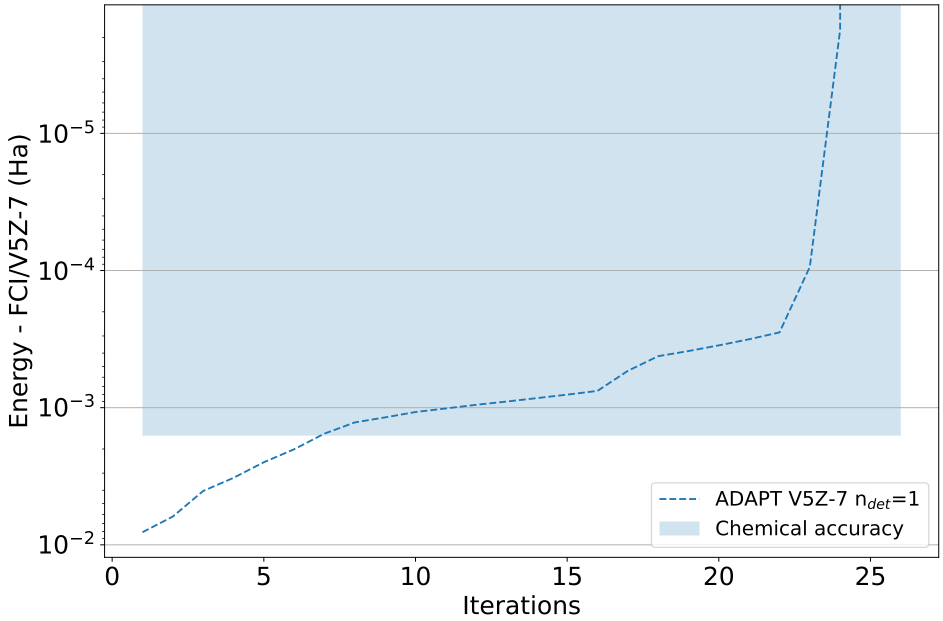


FIG. 8: Error in the ADAPT-VQE energy with respect to the FCI energy with the number of VQE iterations for the LiH molecule with the SABS/V5Z-7 basis. The starting point is the HF determinant. The number of required qubits is 16.

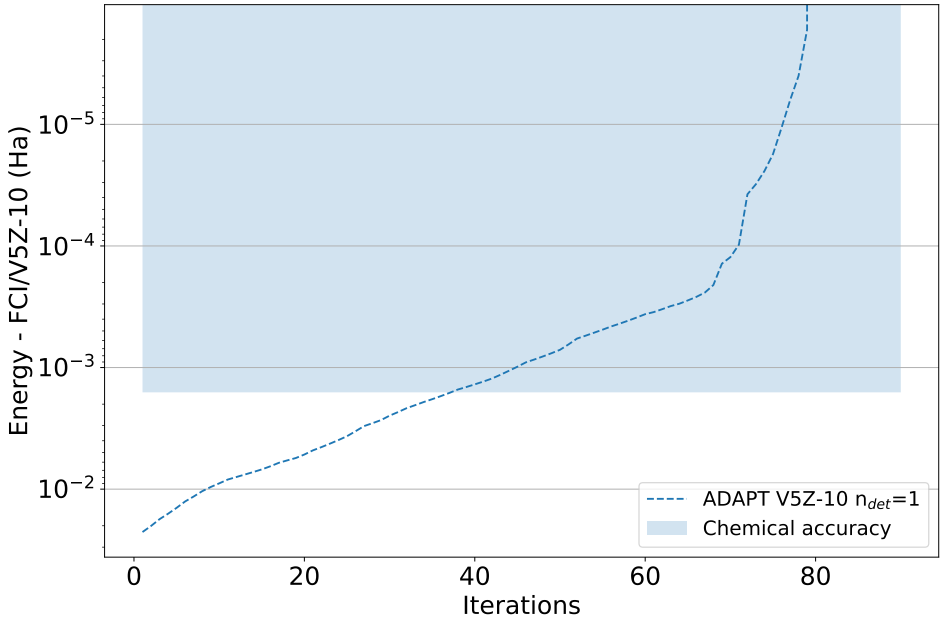


FIG. 9: Error in the ADAPT-VQE energy with respect to the FCI energy with the number of VQE iterations for the LiH molecule with the SABS/V5Z-10 basis set. The starting point is the HF determinant. The number of required qubits is 28.

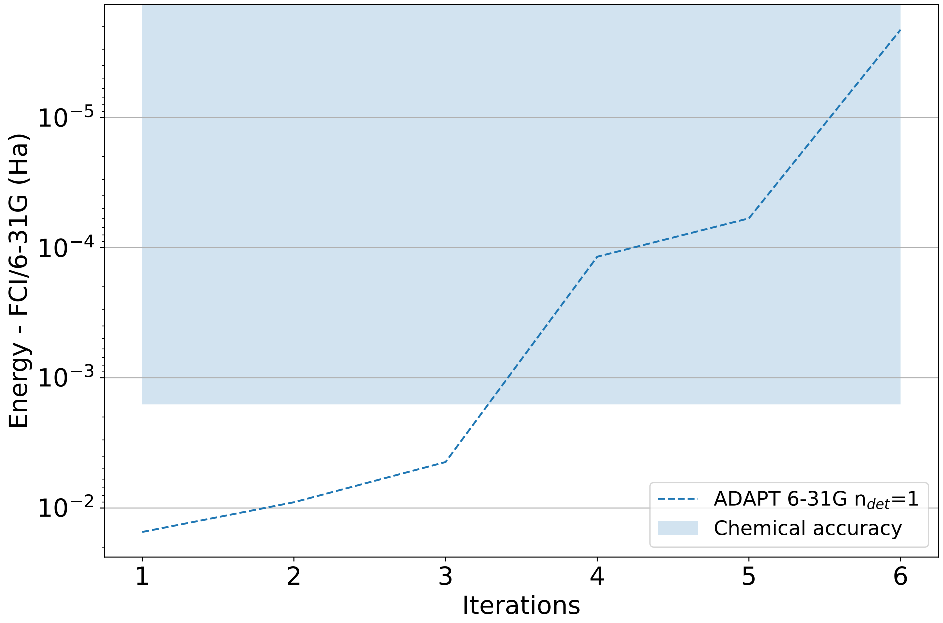


FIG. 10: Error in the ADAPT-VQE energy with respect to the FCI energy with the number of VQE iterations for the $H_2$ molecule with the 6-31G basis set. The starting point is the HF determinant. The number of required qubits is 8.

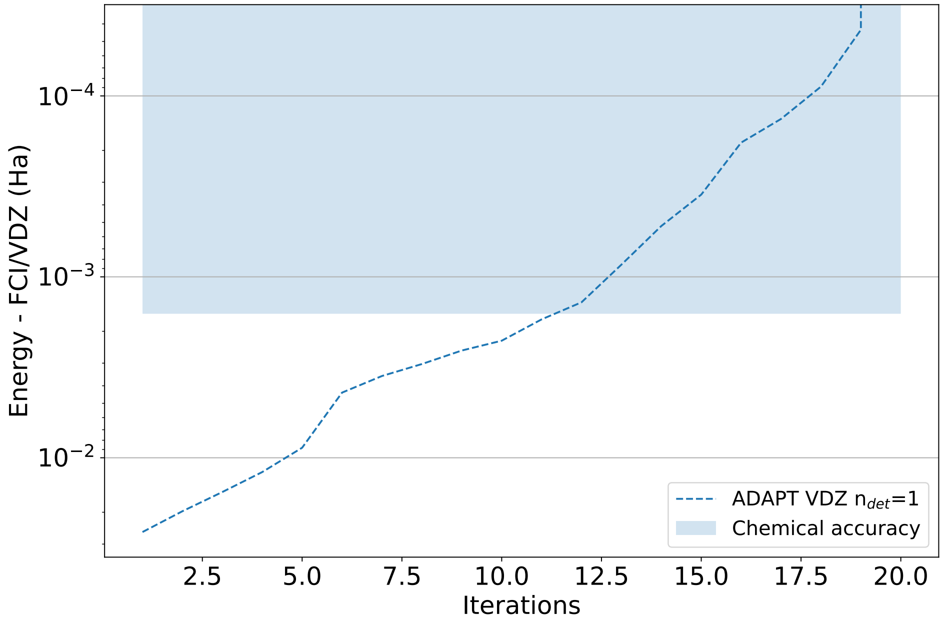


FIG. 11: Error in the ADAPT-VQE energy with respect to the FCI energy with the number of VQE iterations for the $H_2$ molecule with the cc-pVDZ basis set. The starting point is the HF determinant. The number of required qubits is 20.

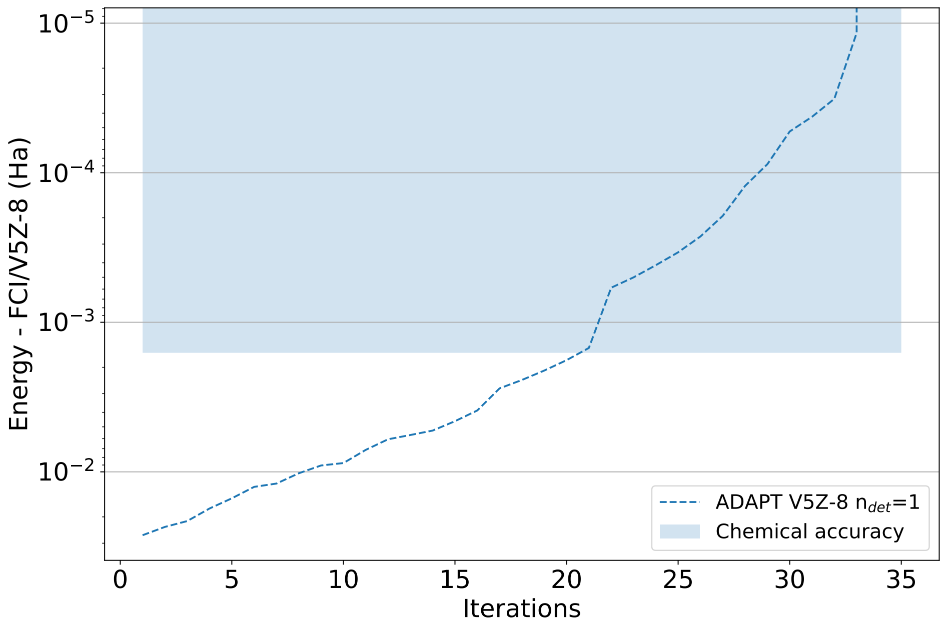


FIG. 12: Error in the ADAPT-VQE energy with respect to the FCI energy with the number of VQE iterations for the $H_2$ molecule with the SABS/V5Z-8. The starting point is the HF determinant. The number of required qubits is 24.

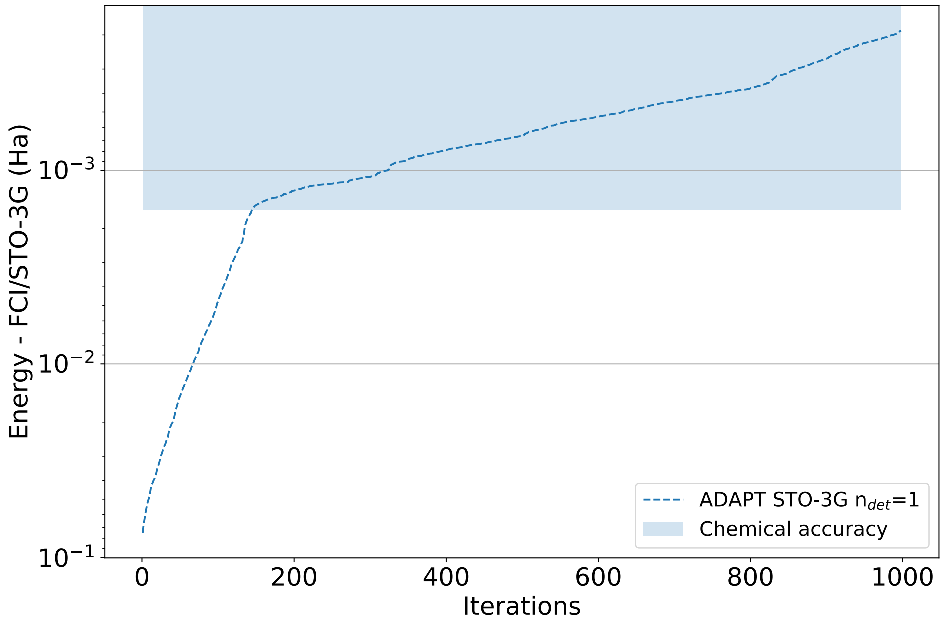


FIG. 13: Error in the ADAPT-VQE energy with respect to the FCI energy with the number of VQE iterations for the $H_8$ molecule with the STO-3G basis set. The starting point is the HF determinant. The number of required qubits is 16.

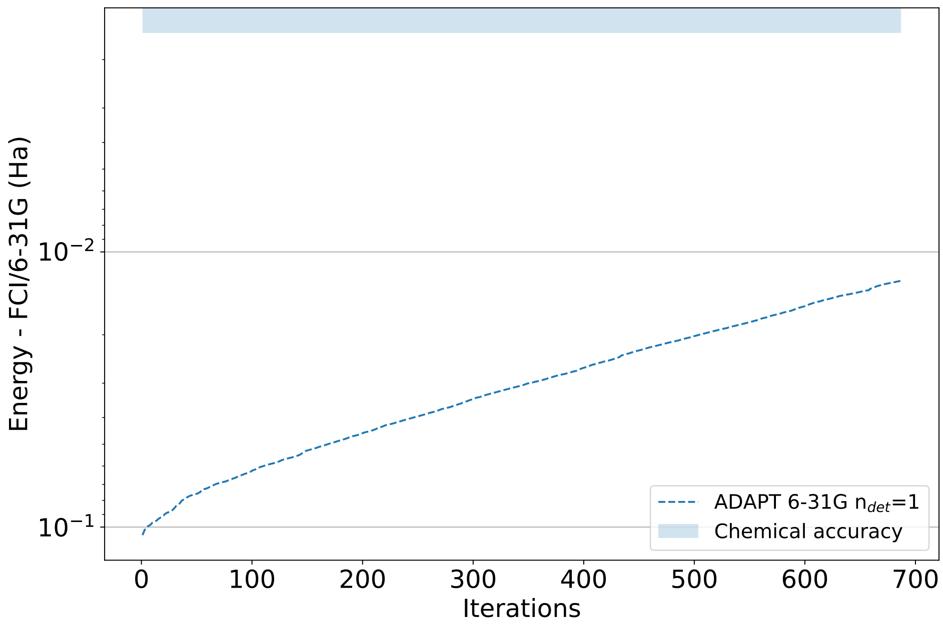


FIG. 14: Error in the ADAPT-VQE energy with respect to the FCI energy with the number of VQE iterations for the $H_8$ molecule with the 6-31G basis-set. The starting point is the HF determinant. The number of required qubits is 32.

[1] P. Jordan and E. P. Wigner, "Über das Paulische äquivalenzverbot," in *The Collected Works of Eugene Paul Wigner*, pp. 109–129, Springer, 1993.

[2] C. D. Batista and G. Ortiz, "Generalized Jordan-Wigner transformations," *Physical Review Letters*, vol. 86, no. 6, p. 1082, 2001.

[3] A. Peruzzo, J. McClean, P. Shadbolt, M.-H. Yung, X.-Q. Zhou, P. J. Love, A. Aspuru-Guzik, and J. L. O'brien, "A variational eigenvalue solver on a photonic quantum processor," *Nature Communications*, vol. 5, no. 1, pp. 1–7, 2014.

[4] A. Y. Kitaev, "Quantum measurements and the abelian stabilizer problem," *Electron. Colloquium Comput. Complex.*, vol. TR96, 1995.

[5] M. A. Nielsen and I. L. Chuang, *Quantum computation and quantum information.* Cambridge University Press, 2010.

[6] A. Aspuru-Guzik, A. D. Dutoi, P. J. Love, and M. Head-Gordon, "Simulated quantum computation of molecular energies," *Science*, vol. 309, no. 5741, pp. 1704–1707, 2005.

[7] J. D. Whitfield, J. Biamonte, and A. Aspuru-Guzik, "Simulation of electronic structure hamiltonians using quantum computers," *Molecular Physics*, vol. 109, no. 5, pp. 735–750, 2011.

[8] J. Tilly, H. Chen, S. Cao, D. Picozzi, K. Setia, Y. Li, E. Grant, L. Wossnig, I. Rungger, G. H. Booth, *et al.*, "The variational quantum eigensolver: a review of methods and best practices," *Physics Reports*, vol. 986, pp. 1–128, 2022.

[9] H. R. Grimsley, S. E. Economou, E. Barnes, and N. J. Mayhall, "An adaptive variational algorithm for exact molecular simulations on a quantum computer," *Nature Communications*, vol. 10, p. 3007, 2019.

[10] C. Feniou, M. Hassan, D. Traoré, E. Giner, Y. Maday, and J.-P. Piquemal, "Overlap-ADAPT-VQE: practical quantum chemistry on quantum computers via overlap-guided compact ansätze," *Communications Physics*, vol. 6, p. 192, jul 2023.

[11] Y. S. Yordanov, V. Armaos, C. H. Barnes, and D. R. Arvidsson-Shukur, "Qubit-excitation-based adaptive variational quantum eigensolver," *Communications Physics*, vol. 4, no. 1, pp. 1–11, 2021.

[12] C. Feniou, M. Hassan, D. Traore, E. Giner, Y. Maday, and J.-P. Piquemal, "Overlap-ADAPT-VQE: Practical Quantum Chemistry on Quantum Computers via Overlap-Guided Compact Ansätze," *Communications Physics*, vol. 6, 2023.

[13] E. Giner, D. Traore, B. Pradines, and J. Toulouse, "Self-consistent density-based basis-set correction: How much do we lower total energies and improve dipole moments?," *Journal of Chemical Physics*, vol. 155, p. 044109, Jul 2021.
